# Supplementary material for: Scaling of Piecewise Deterministic Monte Carlo for Anisotropic Targets
Source: arXiv:2305.00694 ancillary file (2024-10-22)
Supplement: Supplementary file 1 [file Supplement.pdf]

*Submitted to Bernoulli*

# Supplement to "Scaling of piecewise deterministic Monte Carlo for anisotropic targets"

JORIS BIERKENS[1,a], KENGO KAMATANI[2,b] and GARETH O. ROBERTS[3,c]

[1]*Delft Institute of Applied Mathematics,* [a]*joris.bierkens@tudelft.nl*
[2]*Institute of Statistical Mathematics,* [b]*kamatani@ism.ac.jp*
[3]*Department of Statistics, University of Warwick,* [c]*Gareth.O.Roberts@warwick.ac.uk*

Proofs for homogenisation of the Zig-Zag sampler and for averaging of the bouncy particle sampler together with some technical proofs.

*MSC2020 subject classifications:* Primary 65C05; 60J25; secondary 62F15
*Keywords:* Markov process; Monte Carlo methods

## Appendix A: Homogenisation of the Zig-Zag sampler

In this section, we derive the convergence of the Zig-Zag sampler. First, we would like to obtain the limit process by formal argument using the series of equations (14). From the first equation of (14) we get $\mathcal{L}_0 u_0(t,y,v) = 0$, i.e. $u_0(t,y,v)$ lies in the null space of $\mathcal{L}_0$ regarding $t$ and $y_{\mathrm{K}}$ as fixed constants. On the other hand, by Proposition 4.2, $\mathcal{L}_0$ is an ergodic operator as a process of $(y_{\mathrm{L}}, v)$. Therefore, $u_0$ is independent of $(y_{\mathrm{L}}, v)$ and is a function of $y_{\mathrm{K}}$ and $t$ (see Section 4.4 of Pavliotis and Stuart (2008)). From this fact, the second equation of (14) becomes Poisson's equation of $u_1$:

$$(\mathcal{L}_0 u_1)(t,y,v) = -(\Lambda_{\mathrm{K}}^{-1}(Uv)_{\mathrm{K}})^\top \partial_{y_{\mathrm{K}}} u_0(t, y_{\mathrm{K}}). \tag{A.1}$$

Note that $\mathcal{L}_0$ does not affect either $y_{\mathrm{K}}$ or $\partial_{y_{\mathrm{K}}} u_0(t, y_{\mathrm{K}})$. Therefore, the solution of $u_1$ is a linear combination of $\chi_0(y_{\mathrm{L}}, v) = \mathcal{L}_0^{-1} v$ whose existence is guaranteed by Theorem 4.2. Indeed, the solution has an expression

$$u_1(t,y,v) = -(\Lambda_{\mathrm{K}}^{-1}(U\chi_0)_{\mathrm{K}})^\top \partial_{y_{\mathrm{K}}} u_0(t, y_{\mathrm{K}}) = \chi(y_{\mathrm{L}}, v)^\top \partial_{y_{\mathrm{K}}} u_0(t, y_{\mathrm{K}}) \tag{A.2}$$

where the integration constant is omitted here. If we take the expected value with respect to $\mu$ for the third equation of (14), then the term $\mathcal{L}_0 u_2$ vanishes since $\mathcal{L}_0$ is an extended generator of a $\mu$-invariant Markov process by Lemma 4.1. We obtain formally

$$\frac{\mathrm{d}u_0}{\mathrm{d}t}(t, y_{\mathrm{K}}) = \mu(\mathcal{L}_1 u_1(t,y,v)).$$

On the other hand

$$\begin{cases} a_i := v_i (U_{\mathrm{K},\cdot}^\top \Lambda_{\mathrm{K}}^{-1} y_{\mathrm{K}})_i \\ b_i := v_i (U_{\mathrm{L},\cdot}^\top \Lambda_{\mathrm{L}}^{-1} y_{\mathrm{L}})_i \end{cases} \quad \Longrightarrow \quad \mathcal{L}_1 u_1 = (\Lambda_{\mathrm{K}}^{-1}(Uv)_{\mathrm{K}})^\top \partial_{y_{\mathrm{K}}} u_1 + \sum_{i=1}^d a_i\, 1(b_i \geq 0)(\mathcal{F}_i - \mathrm{id}) u_1.$$

By (21), we have

$$\sum_{i=1}^{d}(\mathcal{F}_i - \mathrm{id})(a_i\ 1(b_i \geq 0)) = -\sum_{i=1}^{d} a_i - \sum_{i=1}^{d} a_i 1(b_i = 0)$$

and

$$\sum_{i=1}^{d} a_i = y_{\mathrm{K}}^{\top}(\Lambda_{\mathrm{K}}^{-1}(Uv)_{\mathrm{K}}) \overset{(17)}{=} -y_{\mathrm{K}}^{\top}\mathcal{L}_0\chi.$$

By $\mu$-reversibility of $\mathcal{F}_i$, we have

$$\begin{aligned}\mu(\mathcal{L}_1 u_1) &= \mu((\Lambda_{\mathrm{K}}^{-1}(Uv)_{\mathrm{K}})^{\top}\partial_{y_{\mathrm{K}}} u_1) + \sum_{i=1}^{d}\mu(u_1(\mathcal{F}_i - \mathrm{id})(a_i\ 1(b_i > 0))) \\ &\overset{(17)}{=} -\mu((\mathcal{L}_0\chi)^{\top}\partial_{y_{\mathrm{K}}} u_1) + \mu(y_{\mathrm{K}}^{\top}(\mathcal{L}_0\chi)u_1).\end{aligned}$$

Thus, by the expression (A.2), the differential equation is

$$\frac{\mathrm{d}u_0}{\mathrm{d}t}(t, y_{\mathrm{K}}) \overset{(19)}{=} \frac{1}{2}\left(\mathrm{tr}\left(\Upsilon\ \partial_{y_{\mathrm{K}}}^2 u_0(t, y_{\mathrm{K}})\right) - y_{\mathrm{K}}^{\top}\Upsilon^{\top}\ \partial_{y_{\mathrm{K}}} u_0(t, y_{\mathrm{K}})\right).$$

For a $k \times k$ matrix $A$ and $k \times k$ symmetric matrix $B$, $\mathrm{tr}(AB) = \mathrm{tr}((A + A^{\top})B)/2$. Thus, the above differential equation can also be expressed as

$$\frac{\mathrm{d}u_0}{\mathrm{d}t}(t, y_{\mathrm{K}}) = \frac{1}{2}\left(\mathrm{tr}\left(\Omega\ \partial_{y_{\mathrm{K}}}^2 u_0(t, y_{\mathrm{K}})\right) - y_{\mathrm{K}}^{\top}\Upsilon^{\top}\ \partial_{y_{\mathrm{K}}} u_0(t, y_{\mathrm{K}})\right).$$

This differential equation corresponds to the Ornstein–Uhlenbeck process (18). See Section 3.4 of Pavliotis (2014) for the relationship between the process and the Kolmogorov backward equation.

These formal arguments imply that the process of $(y_{\mathrm{L}}, v)$ moves rapidly on the order of $\epsilon$, and the process of $y_{\mathrm{K}}$ converges to the Ornstein–Uhlenbeck process on the order of $\epsilon^{-1}$. We will confirm these observations in two steps. First we show the convergence of the fast dynamics $(y_{\mathrm{L}}, v)$ where $y_{\mathrm{K}}$ is almost a constant process in this dynamics.

**Theorem A.1 (Faster dynamics).** *Let $\xi_0(t) = (y_0(t), v_0(t))$ be the Markov process that has the extended generator (11) regarding that $y_{\mathrm{K}}$ is a fixed constant. The $\epsilon$-time scaled Markov process $\xi^{\epsilon}(\epsilon t)$ of (10) converges to Markov process $\xi_0(t)$ in the Skorokhod topology where the initial distribution of both of the processes is the stationary distribution $\mathcal{N}_d(0, I_d) \otimes \mathcal{U}(\{-1, +1\}^d)$.*

**Proof.** Let $\xi_*^{\epsilon}(t) = (y_*^{\epsilon}(t), v_*^{\epsilon}(t)) = \xi^{\epsilon}(\epsilon t)$ be the $\epsilon$-time scaled Markov process of (10) corresponding to the extended generator

$$\mathcal{L}_*^{\epsilon} f(y, v) = \epsilon((\Lambda^{\epsilon})^{-1}Uv)^{\top}\partial_y f(y, v) + \epsilon\sum_{i=1}^{d}(v_i(U^{\top}(\Lambda^{\epsilon})^{-1}y)_i)_+\ (\mathcal{F}_i - \mathrm{id})f(y, v).$$

Without loss of generality, we can assume $\xi_*^{\epsilon}(0) = \xi_0(0)$. Throughout in this proof we treat $\xi_0(0)$ as a fixed constant. Since the velocity process $v_*^{\epsilon}(t)$ satisfies $|v_*^{\epsilon}(t)| = \sqrt{d}$, we have a local uniform bound

$$y_*^{\epsilon}(t) = y_0(t) + \epsilon\int_0^t (\Lambda^{\epsilon})^{-1}Uv_*^{\epsilon}(s)\mathrm{d}s \quad\Longrightarrow\quad |y_*^{\epsilon}(t) - y_0(0)| \leq \sqrt{d}\ \|\epsilon\ (\Lambda^{\epsilon})^{-1}\| t.$$

Since $\|\epsilon(\Lambda^\epsilon)^{-1}\| \le \|\Lambda_{\mathrm{K}}^{-1}\| + \|\Lambda_{\mathrm{L}}^{-1}\|$ for $\epsilon \in (0,1]$, it is bounded. Thus the Markov process is bounded on any finite interval $[0,T]$. By a similar argument, $y_0(t)$ is also bounded on any finite interval. Therefore we can apply Theorem IX.3.27 of Jacod and Shiryaev (2003), which is the limit theorem for bounded processes.

Jumps of $\xi_*^\epsilon$ is generated from $v$ and the compensator of the random measure associated to the process $v^\epsilon$ is defined by

$$\int_{\mathbb{R}^{2d}} h(\xi)\nu_t^\epsilon(\mathrm{d}\xi) = \sum_{i=1}^d \int_0^t \lambda_i^\epsilon(\xi_*^\epsilon(s))h(0,(F_i - \mathrm{id})(v_*^\epsilon(s)))\mathrm{d}s$$

where

$$\lambda_i^\epsilon(\xi) = \epsilon\ (v_i(U^\top(\Lambda^\epsilon)^{-1}y)_i)_+.$$

Write $\nu_t$ for the compensator corresponding to $\xi_0$. Since each jump size is always 2,

$$a > 2 \quad\Longrightarrow\quad \int_{\mathbb{R}^{2d}} |\xi|^2 1_{\{|\xi|>a\}}\nu_t^\epsilon(\mathrm{d}\xi) = 0 \quad\Longrightarrow\quad (3.29).$$

Similarly, condition (ii), i.e., 3.28 and condition 3.24 are satisfied. Let

$$b^\epsilon(\xi) := (\mathcal{L}_*^\epsilon\ \mathrm{id})(\xi), \quad B_t'^\epsilon := \int_0^t b^\epsilon(\xi_*^\epsilon(s))\mathrm{d}s,$$
$$b(\xi) := (\mathcal{L}_0\ \mathrm{id})(\xi), \quad B_t' := \int_0^t b(\xi_0(s))\mathrm{d}s$$

where, id is the identity function. Then, by Dynkin's formula, $\xi_*^\epsilon(t) - \xi_*^\epsilon(0) - B_t'^\epsilon$ and $\xi_0(t) - \xi_0(0) - B_t'$ are local martingales. We have

$$b^\epsilon(\xi) = \left(\epsilon(\Lambda^\epsilon)^{-1}Uv, \quad \epsilon\sum_{i=1}^d (v_i(U^\top(\Lambda^\epsilon)^{-1}y)_i)_+(F_i - \mathrm{id})v\right) \quad\longrightarrow_{\epsilon\to 0}$$
$$\left(\left(0, \Lambda_{\mathrm{L}}^{-1}(Uv)_{\mathrm{L}}\right), \quad \sum_{i=1}^d (v_i(U_{\mathrm{L},\cdot}^\top\Lambda_{\mathrm{L}}^{-1}y_{\mathrm{L}})_i)_+(F_i - \mathrm{id})v\right) = b(\xi)$$

locally uniformly in $\xi = (y,v)$. Thus

$$B_t'^\epsilon - B_t' \circ \xi_*^\epsilon \longrightarrow_{\epsilon\to 0} 0 \quad\Longrightarrow\quad [\mathrm{Sup}\text{-}\beta_7']$$

where $B_t' \circ \xi_*^\epsilon$ is the process $B_t'$ replacing $\xi_0$ by $\xi_*^\epsilon$. Similarly,

$$\tilde{C}_t' := \int_{\mathbb{R}^d} v^{\otimes 2}\nu_t(\mathrm{d}v), \quad \tilde{C}_t'^\epsilon = \int_{\mathbb{R}^d} v^{\otimes 2}\nu_t^\epsilon(\mathrm{d}v) \quad \Longrightarrow \tilde{C}_t'^\epsilon - \tilde{C}_t' \circ \xi_*^\epsilon \quad \longrightarrow_{\epsilon\to 0} 0$$
$$\Longrightarrow [\gamma_7'\text{-}\mathrm{D}]$$

where $\tilde{C}_t' \circ \xi_*^\epsilon$ is the process $\tilde{C}_t'$ replacing $\xi_0$ by $\xi_*^\epsilon$. The same convergence holds by replacing $v^{\otimes 2}$ by $g$ where $g : \mathbb{R}^d \to \mathbb{R}$ is a continuous bounded function which is 0 around $0 \in \mathbb{R}^d$. This yields $[\delta_{7,1}\text{-D}]$. Other regularity conditions (i), (iv) and (v) can easily be verified.

Finally we check the condition (iii), uniqueness of the corresponding martingale problem of (23). Since the process has a bounded velocity, it is non-explosive. Also, there exists a solution and the solution has pathwise uniqueness as in Section IV.9 of Ikeda and Watanabe (1989). On the other hand, by state augmentation technique, by Theorem 2.3 of Kurtz (2011), any solution of the martingale problem has a modification with sample paths in $\mathbb{D}_{\mathbb{R}^d\times\mathbb{R}^d}[0,\infty)$. It implies the uniqueness of the martingale problem. Thus the claim follows. □

Our next task is to demonstrate the convergence of the slower dynamics, which corresponds to Theorem 3.2. Let $|||X|||_T = \mathbb{E}[\sup_{0\le t\le T} |X(t)|]$.

**Proof of Theorem 3.2.** Let

$$\xi^\epsilon_\sharp(t) = \xi^\epsilon(\epsilon^{-1}t), \quad z^\epsilon(t) = y^\epsilon_{\mathrm{K}}(\epsilon^{-1}t).$$

Let $\kappa(\xi) = (y_{\mathrm{L}}, v)$. We prove the convergence of the process $z^\epsilon$. For this purpose, it is easier to work on another process $\tilde{z}^\epsilon$ defined by

$$\tilde{z}^\epsilon(t) = z^\epsilon(0) + \int_0^t (-\mathcal{L}^\epsilon + \mathcal{L}_1)(\chi\circ\kappa)(\xi^\epsilon_\sharp(s))\mathrm{d}s + \epsilon\,(\chi\circ\kappa)(\xi^\epsilon_\sharp(t)) \tag{A.3}$$

which has a decomposition $\tilde{z}^\epsilon - \tilde{z}^\epsilon(0) = M^\epsilon + A^\epsilon$ where $M^\epsilon$ is a local martingale defined by

$$M^\epsilon(t) = \epsilon\left\{(\chi\circ\kappa)(\xi^\epsilon_\sharp(t)) - (\chi\circ\kappa)(\xi^\epsilon_\sharp(0)) - \epsilon^{-1}\int_0^t \mathcal{L}^\epsilon(\chi\circ\kappa)(\xi^\epsilon_\sharp(s))\mathrm{d}s\right\} \tag{A.4}$$

and $A^\epsilon$ is a predictable process defined by

$$A^\epsilon(t) = \int_0^t \mathcal{L}_1(\chi\circ\kappa)(\xi^\epsilon_\sharp(s))\mathrm{d}s. \tag{A.5}$$

We show that the gap between $z^\epsilon$ and $\tilde{z}^\epsilon$ is negligible. Since the function $\psi(y,v) = y_{\mathrm{K}}$ does not depend on $y_{\mathrm{L}}$ nor $v$, we have

$$\mathcal{L}^\epsilon\psi(y,v) = \mathcal{L}_1\psi(y,v) \overset{(17)}{=} -\mathcal{L}_0\chi(y_{\mathrm{L}},v).$$

From this equation, we have

$$z^\epsilon(t) - z^\epsilon(0) = \epsilon^{-1}\int_0^t (\mathcal{L}^\epsilon\psi)(\xi^\epsilon_\sharp(s))\mathrm{d}s = -\epsilon^{-1}\int_0^t (\mathcal{L}_0\chi)(\kappa(\xi^\epsilon_\sharp(s)))\mathrm{d}s.$$

Observe that $(\mathcal{L}_0\chi)(\kappa(\xi)) = \mathcal{L}_0(\chi\circ\kappa)(\xi)$ where, in the right-hand side, $\mathcal{L}_0$ operate to $\chi\circ\kappa(y_{\mathrm{K}}, y_{\mathrm{L}}, v)$ regarding $y_{\mathrm{K}}$ as a constant. The difference between $z^\epsilon$ and $\tilde{z}^\epsilon$ is

$$\sup_{0\le t\le T} |z^\epsilon(t) - \tilde{z}^\epsilon(t)| \le \int_0^T \left|(\mathcal{L}^\epsilon - \epsilon^{-1}\mathcal{L}_0 - \mathcal{L}_1)(\chi\circ\kappa)(\xi(t))\right|\mathrm{d}t + \epsilon \sup_{0\le t\le T}|\chi\circ\kappa(\xi^\epsilon_\sharp(t))|.$$

The first term in the right-hand side converges in probability to 0 by Lemma A.2 below and by Lebesgue's dominated convergence theorem. The convergence of the second term will be described in Lemma A.5. Thus $\sup_{0\le t\le T}|z^\epsilon(t) - \tilde{z}^\epsilon(t)| \longrightarrow 0$ in probability.

Now we focus on $\tilde{z}^\epsilon$. We apply Theorem XI.3.48 if Jacod and Shiryaev (2003) to $\tilde{z}^\epsilon$ and check the convergence to the Ornstein–Uhlenbeck process. Conditions (i-v) are satisfied since the limit process is

the Ornstein–Uhlenbeck process. Conditions (vi) [Sup-$\beta'_{\text{loc}}$] and [$\gamma'_{\text{loc}}$-D] will be checked in Lemmas A.3 and A.4. Now we would like to check the condition (vi) [$\delta_{\text{loc}}$-D]. Jumps of $\tilde{z}^{\epsilon}(t)$ are generated from $\epsilon\,(\chi\circ\kappa)(\xi^{\epsilon}_{\sharp}(t))$ and the compensator of the random measure associated to the process is

$$(h*\nu^{\epsilon})(t) := \int_{\mathbb{R}^d\times\mathbb{R}^d} h(\xi)\nu^{\epsilon}_t(\mathrm{d}\xi) := \sum_{i=1}^{d}\int_0^t \lambda^{\epsilon}_i(\xi^{\epsilon}_{\sharp}(s))\; h(0,\epsilon\, J_i(\xi^{\epsilon}_{\sharp}(s))))\mathrm{d}s. \tag{A.6}$$

for $h:\mathbb{R}^d\times\mathbb{R}^d\to\mathbb{R}$ where

$$\lambda^{\epsilon}_i(\xi) := (v_i(U^{\top}(\Lambda^{\epsilon})^{-1}y)_i)_+,\quad J_i(\xi) := (\mathcal{F}_i - \mathrm{id})(\chi\circ\kappa)(\xi).$$

On the other hand the Ornstein–Uhlenbeck process has no jump, that is, the jump component corresponding to the limit process is $\nu\equiv 0$. The class of functions considered in [$\delta_{\text{loc}}$-D] are bounded continuous functions which are zero around the origin. Therefore, it is sufficient to show the following convergence for the indicator function $\delta_a(v,y) = 1(|v|>a)$ for $a>0$:

$$|||\delta_a * \nu^{\epsilon}|||_T \longrightarrow 0.$$

We have

$$|\delta_a(\xi)| \le \left(\frac{|v|}{a}\right)^2 =: \delta_{a,2}(\xi) \quad\Longrightarrow\quad |||\delta_a*\nu^{\epsilon}|||_T \le \left|\left|\left|\delta_{a,2}*\nu^{\epsilon}\right|\right|\right|_T.$$

Furthermore, by stationarity, we have

$$\left|\left|\left|\delta_{a,2}*\nu^{\epsilon}\right|\right|\right|_T \le T\sum_{i=1}^{d}\mathbb{E}\left[\left|\lambda^{\epsilon}_i(\xi)\left(\frac{|\epsilon\, J_i(\xi))|}{a}\right)^2\right|\right] \longrightarrow 0$$

since $|J_i|\le|\chi|+|\mathcal{F}_i\chi|$ has any order of moments, and $\lambda^{\epsilon}_i$ is on the order of $\epsilon^{-1}$. A similar arguments shows the condition IX.3.49. Therefore, $\tilde{z}^{\epsilon}$ converges to the Ornstein–Uhlenbeck process.

From this fact, $z^{\epsilon}$ converges to the same limit process by Lemma VI.3.30 of Jacod and Shiryaev (2003) which completes the proof. □

**Lemma A.2.** *Let $f:\mathbb{R}^d\times\mathbb{R}^d\to\mathbb{R}$ be a differentiable function. For each $\xi=(y,v)$, we have*

$$(\delta f)(\xi) := (\mathcal{L}^{\epsilon} - \epsilon^{-1}\mathcal{L}_0 - \mathcal{L}_1)f(\xi) \longrightarrow_{\epsilon\to 0} 0$$

*pointwise, where we operate $\mathcal{L}_0$ to $f(y_{\mathrm{K}},y_{\mathrm{L}},v)$ regarding $y_{\mathrm{K}}$ as a fixed constant. Also,*

$$|(\delta f)(\xi)| \le 2\sum_{i=1}^{d}\left|(U^{\top}_{\mathrm{K},\cdot}\Lambda^{-1}_{\mathrm{K}}y_{\mathrm{K}})\right|\;(|f(\xi)|+|\mathcal{F}_i f(\xi)|).$$

**Proof.** Observe that

$$a_i := v_i(U^{\top}_{\mathrm{K},\cdot}\Lambda^{-1}_{\mathrm{K}}y_{\mathrm{K}})_i,\ b_i := v_i(U^{\top}_{\mathrm{L},\cdot}\Lambda^{-1}_{\mathrm{L}}y_{\mathrm{L}})_i$$
$$\Longrightarrow (\delta f)(\xi) = \sum_{i=1}^{d}\Big((a_i+\epsilon^{-1}b_i)_+ - \epsilon^{-1}(b_i)_+ - a_i 1(b_i>0)\Big)(\mathcal{F}_i-\mathrm{id})f(\xi).$$

Thus the first claim is a direct consequence of

$$(a+\epsilon^{-1}b)_+ - \epsilon^{-1}b_+ - a\, 1(b>0) \neq 0$$
$$\iff \quad \operatorname{sgn}(a+\epsilon^{-1}b) \neq \operatorname{sgn}(\epsilon^{-1}b) \quad \Longrightarrow \quad |a| > \epsilon^{-1}|b|.$$

Also, from this relation, we have

$$\left|(a+\epsilon^{-1}b)_+ - \epsilon^{-1}b_+ - a\, 1(b>0)\right| \le |a+\epsilon^{-1}b| \le 2|a|.$$

This proves the second claim. □

**Lemma A.3.** *For any $T>0$,*

$$|||C^\epsilon - C|||_T \longrightarrow_{\epsilon\to 0} 0$$

*where $C^\epsilon$ is the predictable quadratic variation of $M^\epsilon$ in (A.4), and $C(t) = t\,\Omega$.*

**Proof.** The martingale $M^\epsilon$ is a purely discontinuous martingale driven by the random measure associated to the jump of $\epsilon\,\chi\circ\kappa(\xi^\epsilon_\sharp(\cdot))$. The random measure has the corresponding compensator $\nu^\epsilon_t$ defined in (A.6). Therefore, the predictable quadratic variation of the martingale $M^\epsilon$ is

$$C^\epsilon(t) = \int_0^t m^\epsilon(\xi^\epsilon_\sharp(s))\mathrm{d}s, \quad m^\epsilon(\xi) = \epsilon\sum_{i=1}^d (v_i(U^\top(\Lambda^\epsilon)^{-1}y)_i)_+ ((\mathcal{F}_i - \mathrm{id})\chi(y_\mathrm{L}, v))^{\otimes 2}$$

by Theorem II.1.33 of Jacod and Shiryaev (2003). This predictable quadratic variation corresponds to the second modified characteristics defined in equation (IX.3.25) of Jacod and Shiryaev (2003). See also Definition II.2.16 and Proposition II.2.17. We set

$$C^\epsilon_0(t) := \int_0^t m(\kappa(\xi^\epsilon_\sharp(s)))\mathrm{d}s$$

where $m(y_\mathrm{L}, v)$ is as in (20). Since $|(a+b)^+ - a^+| \le |b|$, we have

$$\delta^\epsilon(\xi) := |m^\epsilon(\xi) - m(\kappa(\xi))| \ \le\ \epsilon \sum_{i=1}^d |v_i(U^\top_{\mathrm{K},\cdot}\Lambda_\mathrm{K}^{-1}y_\mathrm{K})_i|\ (|\mathcal{F}_i\chi(y_\mathrm{L}, v)| + |\chi(y_\mathrm{L}, v)|)^2. \tag{A.7}$$

Thus we have

$$\left\|C^\epsilon - C^\epsilon_0\right\|_T \le T\,\mathbb{E}[|\delta^\epsilon(\xi^\epsilon(0))|] \quad \overset{(A.7)}{\longrightarrow} \quad 0.$$

Let

$$m_0(y_\mathrm{L}, v) := m(y_\mathrm{L}, v) - \Omega, \quad \overset{\text{Lemma 4.5}}{\Longrightarrow} \quad \mu(m_0) = 0.$$

For $\xi^\epsilon_*(t) = \xi^\epsilon(\epsilon t)$, we have

$$C^\epsilon_0(t) - C(t) = \epsilon^2 \int_0^{\epsilon^{-2}t} m_0(\kappa(\xi^\epsilon_*(t)))\mathrm{d}t.$$

Therefore, by Lemma C.9, for any $S > 0$ we have

$$\begin{aligned} T^{-1} \left\|\!\left| C_0^\epsilon - C \right|\!\right\|_T &\leq \mathbb{E}\left[\frac{1}{S}\left|\int_0^S m_0(\kappa(\xi_*^\epsilon(t)))\mathrm{d}t\right|\right] + \frac{S}{\epsilon^{-2}T}\mu(|m_0|) \\ &\longrightarrow_{\epsilon\to 0} \mathbb{E}\left[\frac{1}{S}\left|\int_0^S m_0(\kappa(\xi_0(t)))\mathrm{d}t\right|\right] \end{aligned}$$

by Proposition A.1 where $\xi_0(t)$ is the process introduced in the proposition. By Proposition 4.2, the process $\xi_0$ is ergodic regarding that $y_{\mathrm{K}}$ is a fixed constant. Thus as $S \longrightarrow \infty$, the right-hand side converges to 0. Thus our claim holds. □

For the Ornstein–Uhlenbeck process (18), let

$$A(t) = \Upsilon \int_0^t X(t)\mathrm{d}t.$$

**Lemma A.4.** *For any $T > 0$, for the process $\tilde{z}^\epsilon$ defined in (A.3) and $A^\epsilon$ defined in (A.5), we have*

$$|||A^\epsilon - A \circ \tilde{z}^\epsilon|||_T \longrightarrow_{\epsilon\to 0} 0.$$

**Proof.** Let

$$\delta(y, v) := (\mathcal{L}_1\chi)(y, v) - \Upsilon\, y_{\mathrm{K}} \implies (A^\epsilon - A \circ z^\epsilon)(t) = \int_0^t \delta(\xi_\sharp^\epsilon(t))\mathrm{d}t.$$

As in the proof of Lemma A.3, by Lemma C.9, for any $S > 0$ we have

$$\lim_{\epsilon\to 0} T^{-1}\, |||A^\epsilon - A \circ z^\epsilon|||_T \leq \mathbb{E}\left[\frac{1}{S}\int_0^S \delta(\xi_0(t))\mathrm{d}t\right]$$

by Proposition A.1 where $\xi_0(t)$ is the process introduced in the proposition. By Proposition 4.2, the process $\xi_0$ is ergodic regarding that $y_{\mathrm{K}}$ is a fixed constant. Thus as $S \longrightarrow \infty$, the right-hand side converges to 0 since $\mu(\delta) = 0$ by Lemma 4.5. Since the gap between $\tilde{z}^\epsilon$ and $z^\epsilon$ is negligible, the claim follows. □

**Lemma A.5.** *For any $T, \delta > 0$, and for $\kappa(\xi) = (y_{\mathrm{L}}, v)$,*

$$\mathbb{P}\left(\epsilon \sup_{0\leq t\leq T} |\chi \circ \kappa(\xi_\sharp^\epsilon(t))| > \delta\right) \longrightarrow_{\epsilon\to 0} 0.$$

**Proof.** By Proposition 4.2, there exists a constant $c_0$ such that $|\chi| = |\Lambda_{\mathrm{K}}^{-1}(U\chi_0)_{\mathrm{K}}| \leq c_0 \exp(|y_{\mathrm{L}}|^2/16\, l^2)$. Thus it is sufficient to show that the event

$$\left\{\sup_{0\leq t<\epsilon^{-1}T} |y_{\mathrm{L}}^\epsilon(t)| > 4l\delta(\epsilon)\right\}$$

is negligible where $\delta(\epsilon) = \sqrt{\log(\epsilon^{-1}c_0^{-1}\delta)}$. On the other hand, there exists $c_1 > 0$ such that $|(y_{\mathrm{L}}^\epsilon)'| = |\epsilon^{-1}\Lambda_{\mathrm{L}}^{-1}(Uv)_{\mathrm{L}}| \leq \epsilon^{-1}c_1$. Therefore, for $h = h(\epsilon) = c_1^{-1}2l\,\epsilon\,\delta(\epsilon)$ we have

$$|y_{\mathrm{L}}^\epsilon(t) - y_{\mathrm{L}}^\epsilon(s)| \leq 2l\delta(\epsilon)$$

if $|t-s| \le h$. From this fact, we have

$$\left\{ \sup_{0\le t<\epsilon^{-1}T} |y^\epsilon_{\mathrm{L}}(t)| > 4l\delta(\epsilon) \right\} \subset \bigcup_{n=1,\dots,[T\epsilon^{-1}/h(\epsilon)]} \left\{ \left|y^\epsilon_{\mathrm{L}}(nh(\epsilon))\right| > 2l\delta(\epsilon) \right\}.$$

Since the process is stationary, and the stationary distribution of $y^\epsilon_{\mathrm{L}}$ is $\mathcal{N}_l(0, I_l)$, we have

$$\begin{aligned}
\mathbb{P}\left( \sup_{0\le t<\epsilon^{-1}T} |y^\epsilon_{\mathrm{L}}(t)| > 4l\delta(\epsilon) \right) &\le [T\epsilon^{-1}/h(\epsilon)]\ \mathbb{P}\left(|y^\epsilon_{\mathrm{L}}(0)| > 2l\delta(\epsilon)\right) \\
&\le [T\epsilon^{-1}/h(\epsilon)]\ \sum_{l\in \mathrm{L}} \mathbb{P}\left(|y^\epsilon_l(0)| > 2\delta(\epsilon)\right) \\
&\le [T\epsilon^{-1}/h(\epsilon)]\ l\ 2\ \Phi(-2\delta(\epsilon))
\end{aligned}$$

where $\Phi(x)$ is the cumulative distribution function of the normal distribution. Since $\Phi(-x) \le \phi(x)$ $(x \ge 1)$, the above probability is dominated above by

$$[T\epsilon^{-1}/h(\epsilon)]\ l\ 2\ \Phi(-2\delta(\epsilon)) = [T\epsilon^{-2}/c_1^{-1} 2l\delta(\epsilon)]\ l\ 2\ (2\pi)^{-1/2} \exp(-2\delta(\epsilon)^2).$$

Since $\exp(-2\delta(\epsilon)^2)$ is on the order of $\epsilon^2$, the right-hand side is on the order of $\delta(\epsilon)^{-1}$. Thus the probability converges to 0. □

## A.1. Proof of Theorem 3.3

For $\lambda^\epsilon_i(y, v) = (v_i(U^\top(\Lambda^\epsilon)^{-1} y)_i)_+$, we derive that

$$\begin{aligned}
\mathbb{E}[N^\epsilon_T] &= \int_0^T \sum_{i=1}^d \mathbb{E}\left[\lambda^\epsilon_i(y^\epsilon(t), v^\epsilon(t)))\right] \mathrm{d}t \\
&= T \sum_{i=1}^d \mathbb{E}\left[\lambda^\epsilon_i(y, v)\right]
\end{aligned}$$

where $(y, v)$ is distributed according to the joint distribution $\mathcal{N}(0, I_d) \otimes \mathcal{U}(\{-1, +1\}^d)$. As the law of $\lambda^\epsilon_i(y, v) + \lambda^\epsilon_i(y, F_i(v)) = |(U^\top(\Lambda^\epsilon)^{-1} y)_i|$ is equivalent to that of $\sqrt{\theta^\epsilon_{i,i}}\ |Z|$ ~~$\sqrt{\Sigma^\epsilon_{i,i}}\ |Z|$~~ where $Z \sim \mathcal{N}(0, 1)$, we conclude that

$$\begin{aligned}
\mathbb{E}[N^\epsilon_T] &= \frac{T}{2} \sum_{i=1}^d \mathbb{E}\left[\lambda^\epsilon_i(y, v) + \lambda^\epsilon_i(y, F_i(v))\right] \\
&= \frac{T}{2} \sum_{i=1}^d \sqrt{\theta^\epsilon_{i,i}}\ \mathbb{E}\left[|Z|\right] \\
&= \frac{T}{2} \sum_{i=1}^d \sqrt{\theta^\epsilon_{i,i}}\ \frac{1}{\sqrt{2\pi}}.
\end{aligned}$$

Given that $(\Sigma^\epsilon)^{-1} = U^\top(\Lambda^\epsilon)^{-2} U = \epsilon^{-2}\Theta_{\mathrm{L}} + O(1)$, the result follows.

# Appendix B: Averaging of the bouncy particle sampler

## B.1. First convergence regime of the bouncy particle sampler

Let $\xi_*^\epsilon(t) = (y_*^\epsilon(t), v_*^\epsilon(t))$ be the $\epsilon$-time scaled Markov process of (12) corresponding to the extended generator

$$\mathcal{L}_*^\epsilon = \epsilon\ ((\Lambda^\epsilon)^{-1}v)^\top\partial_y + \epsilon\ (v^\top(\Lambda^\epsilon)^{-1}y)_+(\mathcal{B}^\epsilon - \mathrm{id}) + \epsilon\ \rho\ (\mathcal{R} - \mathrm{id}).$$

First we prove the convergence $\xi_*^\epsilon \longrightarrow \xi_0$ in Skorokhod topology where $\xi_0(t) = (y_0(t), v_0(t))$ is the Markov process with extended generator (23). We assume that $\xi_0(0) = \xi_*^\epsilon(0)$.

**Proposition B.1 (Fast convergence regime).** *As $\epsilon \to 0$, the Markov process $\xi_*^\epsilon$ starting from $(x, v) \in \mathbb{R}^d \times \mathbb{R}^d$ converges to another Markov process of (23) in Skorokhod topology.*

**Proof.** We assume that $\xi_*^\epsilon(0) = \xi_0(0)$ and consider the initial points as fixed constants. By Lemma VI.3.31, without loss of generality, we can assume that $\rho = 0$, since the refreshment jump occurs in the time interval $[0, T]$ with probability $1 - \exp(-\epsilon\rho T)$, which converges to 0 for $\epsilon \to 0$. The reflection jump does not change the size of the velocity variable, that is, $|v_*^\epsilon(t)| = |v_0(0)|$. Therefore, we have a local uniform bound

$$y_*^\epsilon(t) = y_0(0) + \epsilon \int_0^t (\Lambda^\epsilon)^{-1}v_*^\epsilon(s)\mathrm{d}s \quad\Longrightarrow\quad |y_*^\epsilon(t) - y_0(0)| \le \epsilon\ \|(\Lambda^\epsilon)^{-1}\|\ |v_0(0)|\ t$$
$$\le (\epsilon\|\Lambda_{\mathrm{K}}^{-1}\| + \|\Lambda_{\mathrm{L}}^{-1}\|)\ |v_0(0)|\ t.$$

A similar inequality holds for $\xi_0$. In particular, the Markov processes are bounded on any finite interval $[0, T]$. Therefore, we can apply Theorem IX.3.27 of Jacod and Shiryaev (2003), which is the limit theorem for bounded processes.

By Dynkin's formula, for $h \in C^1(\mathbb{R}^d \times \mathbb{R}^d)$, the compensator associated to the jumps of $\xi_*^\epsilon$ is characterised by

$$\int_{\mathbb{R}^d\times\mathbb{R}^d} h(\xi)\nu_t^\epsilon(\mathrm{d}\xi) := \int_0^t \lambda^\epsilon(\xi_*^\epsilon(s))\ h(0, (\mathcal{B}^\epsilon(y_*^\epsilon(s)) - \mathrm{id})v_*^\epsilon(s))\mathrm{d}s$$

where

$$\lambda^\epsilon(\xi) = \epsilon\ (v^\top(\Lambda^\epsilon)^{-1}y)_+.$$

Write $\nu_t$ for the compensator associated to the jumps of $\xi_0$. Since each jump size is bounded above by $2|v_0(0)|$, we have

$$a > 2|v_0(0)| \implies \int_{\mathbb{R}^d} |v|^2\ 1_{\{|v|>a\}}\nu_t^\epsilon(\{0\}\times\mathrm{d}v) = 0 \implies (3.29).$$

Similarly, condition (ii), i.e., 3.28 and condition 3.24 are satisfied. We have

$$b^\epsilon(\xi) := \Big(\epsilon(\Lambda^\epsilon)^{-1}v, \quad \epsilon\ (v^\top(\Lambda^\epsilon)^{-1}y)_+(B^\epsilon(y) - \mathrm{id})v\Big)$$
$$\longrightarrow_{\epsilon\to 0} \Big(\big(0, \Lambda_{\mathrm{L}}^{-1}v_{\mathrm{L}}\big), \big(0, (v_{\mathrm{L}}^\top\Lambda_{\mathrm{L}}^{-1}y_{\mathrm{L}})_+(B^0(y) - \mathrm{id})v_{\mathrm{L}}\big)\Big) =: b(\xi)$$

locally uniformly in $\xi = (y, v)$. Let

$$B_t'^{\epsilon} := \int_0^t b^\epsilon(\xi_*^\epsilon(s))\mathrm{d}s, \quad B_t' := \int_0^t b(\xi_0(s))\mathrm{d}s.$$

Then

$$B_t'^{\epsilon} - B_t' \circ \xi_*^\epsilon \longrightarrow_{\epsilon\to 0} 0 \implies [\text{Sup}-\beta_7']$$

where $B_t' \circ \xi_*^\epsilon$ is the process $B_t'$ replacing $\xi$ by $\xi_*^\epsilon$. Similarly,

$$\tilde{C}_t' := \int_{\mathbb{R}^d} v^{\otimes 2}\nu_t(\{0\}\times \mathrm{d}v) \quad \implies \quad \tilde{C}_t'^{\epsilon} := \int_{\mathbb{R}^d} v^{\otimes 2}\nu_t^\epsilon(\{0\}\times \mathrm{d}v) \longrightarrow_{\epsilon\to 0} \widetilde{C}_t' \circ \xi_*^\epsilon$$
$$\implies [\gamma_7'\text{–D}]$$

where $\widetilde{C}_t' \circ \xi_*^\epsilon$ is the process $\widetilde{C}_t$ replacing $\xi$ by $\xi_*^\epsilon$. The same convergence holds by replacing $v^{\otimes 2}$ by $g$ where $g : \mathbb{R}^d \to \mathbb{R}$ is a continuous bounded function which is 0 around $0 \in \mathbb{R}^d$. This yields [$\delta_{7,1}$-D]. Other regularity conditions (i), (iv) and (v) can easily be verified.

The argument used in Theorem A.1 is used to establish both the uniqueness of the corresponding martingale problem in equation (23) and condition (iii). □

## B.2. Reparametrisation and expansion of the generator

We contemplate the reparametrisation of $(y, v)$ in order to facilitate the analysis. Let

$$x = (y_\mathrm{K}, v_\mathrm{K}, \alpha, \beta), \quad \zeta = (z, e, x) = (z, e, y_\mathrm{K}, v_\mathrm{K}, \alpha, \beta)$$

and let $\psi, \pi$ be projections such that

$$(y, v) \quad \overset{\pi}{\longrightarrow} \quad \zeta = (z, e, x) \quad \overset{\psi}{\longrightarrow} \quad x = (y_\mathrm{K}, v_\mathrm{K}, \alpha, \beta) \tag{B.1}$$

where $\alpha$ and $\beta$ are as in (24). Let $\Pi$ be the two-dimensional hyperplane spanned by $y_\mathrm{L}(0)$ and $v_\mathrm{L}(0)$. The processes $y_\mathrm{L}(t)$ and $v_\mathrm{L}(t)$ remain on the hyperplane until the next refreshment jump. Let $\gamma \in \{-1, +1\}$ be the orientation of the hyperplane $\Pi$. When $\Pi$ and $\gamma$ are fixed, then $(y, v)$ and $\zeta$ have a one-to-one correspondence. Since $\Pi$ and $\gamma$ are fixed between the refreshment jump times, we focus on the variable $\zeta$. Let $r = \sqrt{\beta/\alpha}$.

We are now going to rewrite the generator $\mathcal{L}^\epsilon$ using the reparametrisation. With the reparametrisation $\pi : (y, v) \mapsto \zeta$ we have the correspondences

$$\begin{cases} y' = (\Lambda^\epsilon)^{-1}v & \mapsto \quad z' = \epsilon^{-1}\alpha^{1/2}, \quad y_\mathrm{K}' = \Lambda_\mathrm{K}^{-1}v_\mathrm{K} \\ (v^\top(\Lambda^\epsilon)^{-1}y)_+ & \mapsto \quad (\epsilon^{-1}\alpha^{1/2}\, z + v_\mathrm{K}^\top\Lambda_\mathrm{K}^{-1}y_\mathrm{K})_+ \\ \mathcal{B}^\epsilon f(\xi) & \mapsto \quad \widetilde{\mathcal{B}}^\epsilon f(\zeta) := \mathcal{B}^\epsilon(f)(\pi^{-1}\zeta) \\ \mathcal{R}f(\xi) & \mapsto \quad \widetilde{\mathcal{R}}f(\zeta) := \mathcal{R}(f)(\pi^{-1}\zeta). \end{cases}$$

The operator $\widetilde{\mathcal{B}}^0$ is given as the pullback of the reflection

$$\zeta = (z, e, x) \mapsto (-z, b(z, e), x).$$

Let $n(v) = v/|v|$ for a vector $v \neq 0$. The refresh operator $\widetilde{\mathcal{R}}$ is given as the jump from $\zeta$ to $\zeta^*$ as follows, where $v^* = (v_{\mathrm{K}}^*, v_{\mathrm{L}}^*) \sim \mathcal{N}(0, I_d)$:

$$\zeta = \begin{pmatrix} z \\ e \\ y_{\mathrm{K}} \\ v_{\mathrm{L}} \\ \alpha \\ \beta \end{pmatrix} \quad \mapsto \quad \zeta^* = \begin{pmatrix} z^* \\ n(w^*) \\ y_{\mathrm{K}} \\ v_{\mathrm{K}}^* \\ |v_{\mathrm{L}}^*|^2 \\ |v_{\mathrm{L}}^*|^2 \, |w^*|^2 - ((v_{\mathrm{L}}^*)^\top w^*)^2 \end{pmatrix} \tag{B.2}$$
$$\text{where } z^* = n(v_{\mathrm{L}}^*)^\top y_{\mathrm{L}}, \quad w^* = (1 - n(v_{\mathrm{L}}^*)\, n(v_{\mathrm{L}}^*)^\top)\, y_{\mathrm{L}}.$$

The generator $\mathcal{L}^\epsilon$ now becomes

$$\mathcal{L}^\epsilon f(z,e,x) = \epsilon^{-1}\alpha^{1/2}\partial_z f(z,e,x) + (\Lambda_{\mathrm{K}}^{-1} v_{\mathrm{K}})^\top \partial_{y_{\mathrm{K}}} f(z,e,x)$$
$$+ (\epsilon^{-1}\alpha^{1/2}\, z + v_{\mathrm{K}}^\top \Lambda_{\mathrm{K}}^{-1} y_{\mathrm{K}})_+ (\widetilde{\mathcal{B}}^\epsilon - \mathrm{id}) f(z,e,x) + \rho\, (\widetilde{\mathcal{R}} - \mathrm{id})(z,e,x).$$

As $\epsilon \longrightarrow 0$ we formally obtain the first order expansion

$$\epsilon\, \mathcal{L}^\epsilon f(z,e,x) \longrightarrow_{\epsilon \to 0} H f(z,e,x).$$

We treat $H$ defined in Section 4.2 of the manuscript~~(26)~~ as an operator on the space of $(z,e,x)$ with a fixed $x$. Furthermore, the formal approximation of the gap $\mathcal{L}^\epsilon - \epsilon^{-1} H$ gives the second order expansion

$$\mathcal{L}_1 f(\zeta) = v_{\mathrm{K}}^\top \Lambda_{\mathrm{K}}^{-1} \partial_{y_{\mathrm{K}}} f(\zeta) + (v_{\mathrm{K}}^\top \Lambda_{\mathrm{K}}^{-1} y_{\mathrm{K}})\, 1(z > 0)(\widetilde{\mathcal{B}}^0 - \mathrm{id}) f(\zeta)$$
$$+ \alpha^{1/2} z_+ \partial \widetilde{\mathcal{B}}^0 f(\zeta) + \rho\, (\widetilde{\mathcal{R}} - \mathrm{id}) f(\zeta) \tag{B.3}$$

where, the operator $\partial \widetilde{\mathcal{B}}^0$ is formally defined by

$$\partial \widetilde{\mathcal{B}}^0 f(\zeta) = \lim_{\epsilon \to 0} \frac{\widetilde{\mathcal{B}}^\epsilon f(\zeta) - \widetilde{\mathcal{B}}^0 f(\zeta)}{\epsilon}. \tag{B.4}$$

The expansion gives $\mathcal{L}^\epsilon = \epsilon^{-1} H + \mathcal{L}_1 + o(\epsilon)$.

**Proposition B.2.** *For each $\zeta = (z,e,x)$, and for the projection $\psi$ defined in (B.1), if $|y_{\mathrm{L}}|^2 = \beta/\alpha + z^2 \neq 0$, we have*

$$(\delta\psi)(\zeta) := (\mathcal{L}^\epsilon - \epsilon^{-1} H - \mathcal{L}_1)\psi(\zeta) \longrightarrow_{\epsilon \to 0} 0$$

*pointwise. Also, if $0 \leq \epsilon \leq 1$, $|(\delta\psi)(\zeta)|$ is uniformly integrable.*

**Proof.** We prepare temporary notation

$$a = (v_{\mathrm{K}}^\top \Lambda_{\mathrm{K}}^{-1} y_{\mathrm{K}}), \; b = (v_{\mathrm{L}}^\top y_{\mathrm{L}}) = \alpha^{1/2} z, \; A = |\Lambda_{\mathrm{K}}^{-1} y_{\mathrm{K}}|, \; B = |y_{\mathrm{L}}|.$$

Since $x$ is treated as a constant for $H$, we have $H\,\psi = 0$. From this, we have an expression

$$(\delta\psi)(\zeta) = \left[ (a + \epsilon^{-1} b)_+ (\widetilde{\mathcal{B}}^\epsilon - \mathrm{id}) - b_+ (\partial \widetilde{\mathcal{B}}^0) \right] \psi(\zeta).$$

Also, since $x$ is not affected by the reflection $\widetilde{\mathcal{B}}^0$, we have $\widetilde{\mathcal{B}}^0\psi(\zeta) = \psi(\zeta)$. This gives an inequality

$$|(\delta\psi)(\zeta)| \le |((a+\epsilon^{-1}b)_+ - \epsilon^{-1}b_+ - a1(b>0))(\widetilde{\mathcal{B}}^\epsilon - \widetilde{\mathcal{B}}^0)\psi(\zeta)| \tag{B.5}$$

$$+ |a1(b>0)(\widetilde{\mathcal{B}}^\epsilon - \widetilde{\mathcal{B}}^0)\psi(\zeta)| \tag{B.6}$$

$$+ b_+ \left|\left(\epsilon^{-1}(\widetilde{\mathcal{B}}^\epsilon - \widetilde{\mathcal{B}}^0) - \partial\widetilde{\mathcal{B}}^0\right)\psi(\zeta)\right|. \tag{B.7}$$

As in the proof of Lemma A.2, the quantity (B.5) converges to 0. Also, (B.6) converges to 0 since $v^\epsilon \longrightarrow v^0$. Now we focus on (B.7). The original parametrisation $(y, v) = \pi^{-1}\zeta$ suits to the estimate of the term. Let $v^\epsilon := B^\epsilon(y)v$. With the notation, we have

$$v^\epsilon = v - 2\frac{\epsilon a + b}{\epsilon^2 A^2 + B^2}\begin{pmatrix}\epsilon\Lambda_{\mathrm{K}}^{-1} y_{\mathrm{K}} \\ y_{\mathrm{L}}\end{pmatrix} \implies$$

$$\partial v^\epsilon = -2\frac{\epsilon a + b}{\epsilon^2 A^2 + B^2}\begin{pmatrix}\Lambda_{\mathrm{K}}^{-1} y_{\mathrm{K}} \\ 0\end{pmatrix} - 2\left(\frac{a}{\epsilon^2 A^2 + B^2} - \frac{2\epsilon A^2(\epsilon a + b)}{(\epsilon^2 A^2 + B^2)^2}\right)\begin{pmatrix}\epsilon\Lambda_{\mathrm{K}}^{-1} y_{\mathrm{K}} \\ y_{\mathrm{L}}\end{pmatrix}.$$

We define

$$\tilde{\psi}(y, v) := (\psi \circ \pi)(y, v) = x.$$

Then we can rewrite the deviation of $\widetilde{\mathcal{B}}^\epsilon$ at $\epsilon = 0$ by the original parametrisation as follows:

$$\epsilon^{-1}(\widetilde{\mathcal{B}}^\epsilon - \widetilde{\mathcal{B}}^0)\psi(\zeta) = \epsilon^{-1}(\tilde{\psi}(y, v^\epsilon) - \tilde{\psi}(y, v^0)) = (\partial_v\tilde{\psi})(y, v^\kappa)\partial v^\kappa \tag{B.8}$$

for some $0 \le \kappa \le \epsilon$. This term converges to $\partial\widetilde{\mathcal{B}}^0\psi(\zeta) = (\partial_v\tilde{\psi})(y, v^0)\partial v^0$ when $\epsilon \longrightarrow 0$ which shows the convergence of (B.7). This completes the proof of the first claim of the proposition.

Now we quantify $|(\delta\psi)(\zeta)|$ by using the decomposition (B.5-B.7). We have

$$|\widetilde{\mathcal{B}}^\epsilon\tilde{\psi}(y, v)| \le \sup_{|v^*| \le |v|} |\tilde{\psi}(y, v^*)| \le |y| + |v| + |v|^2 + |y|^2|v|^2 =: \psi^* \implies (B.5) + (B.6) \le 4|a|\,\psi^*.$$

Next we quantify (B.7) by using (B.8). By construction,

$$\partial_v\tilde{\psi}(y, v) = \begin{pmatrix} 0 & 0 \\ I_{\mathrm{K}} & 0 \\ 0 & 2v_{\mathrm{L}} \\ 0 & 2|y_{\mathrm{L}}|^2\, v_{\mathrm{L}} - 2(y_{\mathrm{L}}^\top v_{\mathrm{L}})y_{\mathrm{L}} \end{pmatrix} \implies |\partial_v\tilde{\psi}(y, v)| \le k + 2|v| + 4|y_{\mathrm{L}}|^2|v|.$$

Thus the proof will be completed if $b\,\partial v^\kappa$ is uniformly integrable. Since $|a| \le A|v_{\mathrm{K}}|, |b| \le B|v_{\mathrm{L}}|$, with some algebra, we have

$$\max\{\epsilon\,|a|, |b|,\ |\epsilon a + b|\} \le |v|\sqrt{\epsilon^2 A^2 + B^2}$$

$$\implies |b(\partial v^\epsilon)_{\mathrm{K}}| = \left|2\,\frac{b\,(\epsilon a + b)}{\epsilon^2 A^2 + B^2} - 2\frac{\epsilon a\, b}{\epsilon^2 A^2 + B^2} + 4\,\frac{\epsilon^2 A^2 b\,(\epsilon A + b)}{(\epsilon^2 A^2 + B^2)^2}\right| A \le 8|v|^2\,A,$$

$$|b(\partial v^\epsilon)_{\mathrm{L}}| = \left|-2\frac{a\,b\,B}{\epsilon^2 A^2 + B^2} + 4\,\frac{\epsilon A^2\,b\,B(\epsilon A + b)}{(\epsilon^2 A^2 + B^2)^2}\right| \le 6|v|^2\,A.$$

Thus the bound can be obtained. □

### B.3. Slower dynamics of the bouncy particle sampler

Let $u = u_0 + \epsilon u_1 + o(\epsilon)$ be the solution of the backward Kolmogorov equation corresponds to the extended generator $\mathcal{L}^\epsilon = \epsilon^{-1} H + \mathcal{L}_1 + o(\epsilon)$. The expansion gives

$$\frac{\mathrm{d}u}{\mathrm{d}t} = \mathcal{L}^\epsilon u \quad \Longrightarrow \quad \begin{cases} Hu_0 & = 0 \\ Hu_1 & = \dfrac{\mathrm{d}u_0}{\mathrm{d}t} - \mathcal{L}_1 u_0 \end{cases}. \tag{B.9}$$

From the first equation on the right hand side, $u_0$ is situated within the null space of $H$. As $H$ serves as the generator for an ergodic Markov process on the space of $(z, e)$, the function within the null space is a constant function with respect to $(z, e)$, that is, $u_0 = u_0(x, t)$. Refer to Section 4.4 of Pavliotis and Stuart (2008). Let $\mu(\mathrm{d}z, \mathrm{d}e) = \mathcal{N}(0, 1) \otimes \mathcal{U}(\mathbb{S})$ be the invariant probability measure corresponding to $H$. In equation (B.9), we can find an ordinary differential equation by taking the expected value with respect to $\mu$. Since $\mu(Hu_1) = 0$, the resulting equation is:

$$\frac{\mathrm{d}u_0}{\mathrm{d}t}(x, t) = \int_{\mathbb{R}\times\mathbb{S}} (\mathcal{L}_1 u_0)(z, e, x, t)\mu(\mathrm{d}z, \mathrm{d}e) =: \mathcal{L}u_0(x, t), \tag{B.10}$$

where we consider $\mathcal{L}$ as an operator for functions of $x$. Observe that $\tilde{\mathcal{B}}^0 f(x) = f(x)$. We can express $\partial\tilde{\mathcal{B}}^0$ using the notation in the proof of Proposition B.2:

$$\partial\tilde{\mathcal{B}}^0 f(x) = \left[(\partial v^0)_{\mathrm{K}}^\top \partial_{v_{\mathrm{K}}} + 2(v_{\mathrm{L}}^0)^\top (\partial v^0)_{\mathrm{L}} \partial_\alpha + 2(|y_{\mathrm{L}}|^2 v_{\mathrm{L}}^0 - (y_{\mathrm{L}}^\top v_{\mathrm{L}}^0) y_{\mathrm{L}})^\top (\partial v^0)_{\mathrm{L}} \partial_\beta\right] f(x).$$

The last part of the right-hand side is 0 since $|y_{\mathrm{L}}|^2 v_{\mathrm{L}} - (y_{\mathrm{L}}^\top v_{\mathrm{L}}) y_{\mathrm{L}}$ and $(\partial v^0)_{\mathrm{L}} \propto y_{\mathrm{L}}$ are orthogonal. We get

$$\begin{aligned}\partial\tilde{\mathcal{B}}^0 f(x) &= -2\frac{(v_{\mathrm{L}} y_{\mathrm{L}})^2}{|y_{\mathrm{L}}|^2} y_{\mathrm{K}}^\top \Lambda_{\mathrm{K}}^{-1} \partial_{v_{\mathrm{K}}} f(x) - 4\left(v_{\mathrm{L}} - 2\frac{v_{\mathrm{L}}^\top y_{\mathrm{L}}}{|y_{\mathrm{L}}|^2} y_{\mathrm{L}}\right)^\top y_{\mathrm{L}} \frac{(v_{\mathrm{K}}^\top \Lambda_{\mathrm{K}}^{-1} y_{\mathrm{K}})}{|y_{\mathrm{L}}|^2} \partial_\alpha f(x) \\ &= -\frac{(v_{\mathrm{L}} y_{\mathrm{L}})^2}{|y_{\mathrm{L}}|^2} \left\{2 y_{\mathrm{K}}^\top \Lambda_{\mathrm{K}}^{-1} \partial_{v_{\mathrm{K}}} f(x) - 4(v_{\mathrm{K}}^\top \Lambda_{\mathrm{K}}^{-1} y_{\mathrm{K}}) \partial_\alpha f(x)\right\}.\end{aligned}$$

Using the expression (B.3), we can write the operator $\mathcal{L}$ as:

$$\mathcal{L}f(x) = \left[v_{\mathrm{K}}^\top \Lambda_{\mathrm{K}}^{-1} \partial_{y_{\mathrm{K}}} - c(\alpha, \beta)\ (2 y_{\mathrm{K}}^\top \Lambda_{\mathrm{K}}^{-1} \partial_{v_{\mathrm{K}}} - 4 y_{\mathrm{K}}^\top \Lambda_{\mathrm{K}}^{-1} v_{\mathrm{K}} \partial_\alpha) + \rho\ (\mathcal{R}^* - \mathrm{id})\right] f(x) \tag{B.11}$$

where $c(\alpha, \beta)$ is the integral of $(v_{\mathrm{L}}^\top y_{\mathrm{L}})^2 / |y_{\mathrm{L}}|^2$ defined in (29). Here the refresh operator $\mathcal{R}^*$ is

$$x = (y_{\mathrm{K}}, v_{\mathrm{K}}, \alpha, \beta) \quad \mapsto \quad x^* = (y_{\mathrm{K}}, v_{\mathrm{K}}^*, |v_{\mathrm{K}}^*|^2, |v_{\mathrm{L}}^*|^2\ (r^2 + z^2)\ u),$$

where $v_{\mathrm{K}}^* \sim \mathcal{N}(0, I_{\mathrm{K}})$, $v_{\mathrm{L}}^* \sim \mathcal{N}(0, I_{\mathrm{L}})$, $z \sim \mathcal{N}(0, 1)$ and $u \sim \mathcal{B}e((l-1)/2, 1/2)$. Here, $u$ corresponds to $1 - (n(v_{\mathrm{L}}^*)^\top n(y_{\mathrm{L}}))^2$ in the notation in (B.2).

The Markov process $X(t) = (y_{\mathrm{K}}(t), v_{\mathrm{K}}(t), \alpha(t), \beta(t))$ corresponding to $\mathcal{L}$ is described as follows. Note that the behaviour of $\alpha(t)$ is characterised by that of $v_{\mathrm{K}}(t)$ between the refreshment jumps. Let $T_0 = 0$, and $T_1, T_2, \ldots$ be jump times of the Poisson process $N_t$ with $\mathbb{E}[N_t] = \rho^{-1} t$. For each $i = 0, 1, \ldots,$

let

$$\begin{cases} y'_{\mathrm{K}}(t) & = \Lambda_{\mathrm{K}}^{-1} v_{\mathrm{K}}(t) \\ v'_{\mathrm{K}}(t) & = -2\, c(\alpha(t), \beta(T_i))\ \Lambda_{\mathrm{K}}^{-1} y_{\mathrm{K}}(t) \\ \alpha(t) & = \alpha(T_i) + |v_{\mathrm{K}}(T_i)|^2 - |v_{\mathrm{K}}(t)|^2 \\ \beta(t) & = \beta(T_i) \end{cases} \tag{B.12}$$

for $T_i \le t < T_{i+1}$. At the refreshment time $T_i$, $y_{\mathrm{K}}(T_i) = y_{\mathrm{K}}(T_i-)$ and other variables are refreshed by the operator $\mathcal{R}^*$. Processes $\xi^\epsilon$ and $X^\epsilon$ are defined by

$$(y^\epsilon(t), v^\epsilon(t)) \xrightarrow{\pi} \xi^\epsilon(t) = (z^\epsilon(t), e^\epsilon(t), X^\epsilon(t)) \xrightarrow{\psi} X^\epsilon(t) = (y^\epsilon_{\mathrm{K}}(t), v^\epsilon_{\mathrm{K}}(t), \alpha^\epsilon(t), \beta^\epsilon(t)).$$

Next we prove the slower dynamics of BPS, which corresponds to Theorem 3.4. The theorem states that as $\epsilon \longrightarrow 0$, the process $X^\epsilon$ converges to $X$ in Skorokhod topology.

**Proof of Theorem 3.4.** We apply Theorem IX.3.39 of Jacod and Shiryaev (2003). First we check three conditions in (vi) of Theorem IX.3.39. Let

$$\begin{cases} b^\epsilon(\xi) := \mathcal{L}^\epsilon \psi(\xi) \\ b(x) \ := \mathcal{L}\ \mathrm{id}(x) \end{cases} \quad \Longrightarrow \quad \begin{cases} B'^{\epsilon}_t := \displaystyle\int_0^t b^\epsilon(\xi^\epsilon(s))\mathrm{d}s \\ B'_t \ := \displaystyle\int_0^t b(X(s))\mathrm{d}s. \end{cases} \tag{B.13}$$

Lemma B.3 shows [Sup-$\beta_{\mathrm{loc}}$], that is, $\sup_{0\le t\le T} |B'^{\epsilon}_t - B'_t \circ X^\epsilon| \longrightarrow 0$ in probability. Also, let

$$\begin{cases} c^\epsilon(\xi) = (v^\top(\Lambda^\epsilon)^{-1}y)_+((\widetilde{\mathcal{B}}^\epsilon - \mathrm{id})\psi)^{\otimes 2}(\xi) + \rho\ \widetilde{\mathcal{R}}[(\psi(\cdot) - \psi(\xi))^{\otimes 2}](\xi) \\ c(x) \ = \rho\ \widetilde{\mathcal{R}}^*[(\cdot - x)^{\otimes 2}](x) \end{cases}$$

$$\Longrightarrow \begin{cases} \tilde{C}'^{\epsilon}_t = \displaystyle\int_0^t c^\epsilon(\xi^\epsilon(s))\mathrm{d}s \\ \tilde{C}'_t \ = \displaystyle\int_0^t c(X(s))\mathrm{d}s. \end{cases}$$

Lemma B.4 shows the condition [$\delta_{\mathrm{loc}}$-D], that is, $\tilde{C}'^{\epsilon}_t - \tilde{C}'_t \circ X^\epsilon \longrightarrow 0$ in probability. For a smooth and bounded function $g : \mathbb{R}^d \to \mathbb{R}_+$ such that $g(x) = 0$ around $x = 0$, and for $\lambda^\epsilon(\xi) = (v^\top(\Lambda^\epsilon)^{-1}y)_+$, set

$$\begin{cases} (J^\epsilon g)(\xi) & = \lambda^\epsilon(\xi)\ g((\widetilde{\mathcal{B}}^\epsilon - \mathrm{id})\psi(\xi)) + \rho\ \widetilde{\mathcal{R}}(g(\psi(\cdot) - \psi(\xi)))(\xi) \\ (J^* g)(x) & = \rho\ \widetilde{\mathcal{R}}^*(g(\cdot - x))(x) \end{cases}$$

$$\Longrightarrow \begin{cases} g * \nu^\epsilon_t & = \displaystyle\int_0^t (J^\epsilon g)(\xi^\epsilon(s))\mathrm{d}s \\ g * \nu_t & = \displaystyle\int_0^t (J^* g)(x(s))\mathrm{d}s. \end{cases}$$

There is a constant $a, b > 0$ such that $g(x) \le a\ 1(|x| > b)$. Thus $g(x) \le a(|x|/b)^2$ and

$$\mathbb{E}\left[\left|\lambda^\epsilon(\xi) g((\widetilde{\mathcal{B}}^\epsilon - \mathrm{id})\psi(\xi))\right|\right] \le a\ \mathbb{E}\left[\left|\lambda^\epsilon(\xi) \frac{|(\widetilde{\mathcal{B}}^\epsilon - \mathrm{id})\psi(\xi)|^2}{b^2}\right|\right].$$

The right-hand side converges to 0 as in (B.14). On the other hand, observe that

$$h(\xi) := \rho\, \widetilde{\mathcal{R}}(g(\psi(\cdot) - \psi(\xi)))(\xi) \Longrightarrow \int_{\mathbb{R}\times\mathbb{S}} h(z,e,x)\mu(\mathrm{d}z,\mathrm{d}e) = (J^* g)(x).$$

By Lemma C.9, for any $0 \le S, T$, and for $\delta = h(\xi) - (J^* g)(\psi(\xi))$, we have

$$\mathbb{E}\left[\left|\frac{1}{T}\int_0^T \delta(\xi^\epsilon(t))\mathrm{d}t\right|\right] \le \mathbb{E}\left[\left|\frac{1}{\epsilon\, S}\int_0^{\epsilon\, S} \delta(\xi^\epsilon(t))\mathrm{d}t\right|\right] = \mathbb{E}\left[\left|\frac{1}{S}\int_0^{S} \delta(\xi^\epsilon(\epsilon t))\mathrm{d}t\right|\right]$$

by integrability of $\delta$. Since $\xi^\epsilon(\epsilon t)$ weakly converges to $\xi(t)$ by Proposition B.1, the right-hand side converges to

$$\mathbb{E}\left[\left|\frac{1}{S}\int_0^{S} \delta(\xi(t))\mathrm{d}t\right|\right].$$

However, since the process is ergodic as a process of $(z, e)$, it converges to 0 by the law of large numbers as $S \longrightarrow +\infty$. This proves $[\delta_{\mathrm{loc}}\text{-D}]$, and hence condition (vi).

Other conditions are easy to check. Hence the claim. □

**Lemma B.3.** *For any $T > 0$, we have $\sup_{0\le t\le T} |B_t'^\epsilon - (B' \circ X^\epsilon)_t| \longrightarrow_{\epsilon\to 0} 0$ in probability, where $B'^\epsilon$ and $B'$ are defined in (B.13).*

**Proof.** Let $b^0(\xi) = \mathcal{L}_1\psi(\xi)$. By Proposition B.2 together with stationarity of the process $\xi^\epsilon$, we have

$$\sup_{0\le t\le T}\left|\int_0^t (b^\epsilon - b^0)(\xi^\epsilon(s))\mathrm{d}s\right| \longrightarrow_{\epsilon\to 0} 0$$

in probability. On the other hand, by the weak law of large numbers,

$$\mathbb{E}\left[\int_0^T (b^0 - b\circ\psi)(\xi^\epsilon(s))\mathrm{d}s\right] \longrightarrow 0$$

as in the previous proof. Thus the claim follows. □

**Lemma B.4.** *For any $T > 0$, we have $\langle M^\epsilon\rangle(T) - C(T) \to 0$.*

**Proof.** We use the same notation as in the proof of Proposition B.2. Let

$$c(\xi) = \rho\, \mathcal{R}[(\psi(\cdot) - \psi(\xi))^{\otimes 2}](\xi), \quad c_b^\epsilon(\xi) = (v^\top(\Lambda^\epsilon)^{-1}y)^+[(\mathcal{B}^\epsilon - \mathcal{B}^0)\psi(\xi)]^{\otimes 2}.$$

$$c^*(x) = \rho\, \widetilde{\mathcal{R}}^*[(\cdot - x)^{\otimes 2}](x) = \int_{\mathbb{R}\times\mathbb{S}} c(z,e,x)\mu(\mathrm{d}z,\mathrm{d}e).$$

We have

$$\langle M^\epsilon\rangle(T) = \int_0^T (c + c_b^\epsilon)(\xi^\epsilon(s))\mathrm{d}s.$$

The contribution of $c_b^\epsilon$ is negligible since

$$\mathbb{E}[|c_b^\epsilon(\xi)|] \le \epsilon\, \mathbb{E}[(\epsilon\, v^\top(\Lambda^\epsilon)^{-1}y)^2]^{1/2}\, \mathbb{E}[|\epsilon^{-1}(\mathcal{B}^\epsilon - \mathcal{B}^0)\phi(\xi)|^4]^{1/2}. \tag{B.14}$$

and the both expectations in the right-hand side is on the order of $O(1)$. Also, as in the proof of Lemma B.3, by the weak law of large numbers, the claim follows. □

## B.4. Proof of Theorem 3.5

For $\lambda^\epsilon(y,v) = (v^\top(\Lambda^\epsilon)^{-1}y)_+ + \rho$, as in the Zig-Zag sampler case, we derive that

$$\mathbb{E}[N_T^\epsilon] = \int_0^T \mathbb{E}\left[\lambda^\epsilon(y^\epsilon(t), v^\epsilon(t)))\right] \mathrm{d}t = T\,\mathbb{E}\left[\lambda^\epsilon(y,v)\right].$$

where $(y,v)$ is distributed according to the joint standard normal distribution. The property $\lambda^\epsilon(y,v) + \lambda^\epsilon(y,-v) = |v^\top(\Lambda^\epsilon)^{-1}y| + 2\rho$ simplifies our calculation, and we have

$$\begin{aligned}\mathbb{E}[N_T^\epsilon] &= \frac{T}{2}\,\mathbb{E}\left[\lambda^\epsilon(y,v) + \lambda^\epsilon(y,-v)\right]\\ &= \frac{T}{2}\,\mathbb{E}\left[|v^\top(\Lambda^\epsilon)^{-1}y| + 2\rho\right]\\ &\le \frac{T}{2}\,\left(\mathbb{E}\left[|(\Lambda^\epsilon)^{-1/2}Z|^2\right] + 2\rho\right) = \frac{T}{2}(\mathrm{diag}((\Lambda^\epsilon)^{-1}) + 2\rho)\end{aligned}$$

where $Z$ is normally distributed. Since $\Lambda^\epsilon = \mathrm{diag}(\Lambda_{\mathrm{K}}, \epsilon\,\Lambda_{\mathrm{L}})$, as $\epsilon$ approaches zero, we obtain the limit

$$\epsilon\,\mathbb{E}[N_T^\epsilon] = \epsilon\,\frac{T}{2}\,\mathbb{E}\left[|v^\top(\Lambda^\epsilon)^{-1}y| + 2\rho\right] \quad \longrightarrow_{\epsilon\to 0} \quad \frac{T}{2}\,\mathbb{E}\left[|v_{\mathrm{L}}^\top(\Lambda_{\mathrm{L}})^{-1}y_{\mathrm{L}}|\right].$$

Since we assumed that $\Lambda_{\mathrm{L}} = I_l$, the above limit is

$$\frac{T}{2}\,\mathbb{E}\left[|v_{\mathrm{L}}^\top\, y_{\mathrm{L}}|\right] = \frac{T}{2}\,\mathbb{E}\left[X\right]\;\mathbb{E}\left[|Y|\right]$$

where $X = |v_{\mathrm{L}}|$ and $Y = (v_{\mathrm{L}}/|v_{\mathrm{L}}|)^\top\, y_{\mathrm{L}} \sim \mathcal{N}(0,1)$ are independent. Given that $X$ and $|Y|$ are the $\chi$-distributed with $l$ and 1 degrees of freedom, respectively, and that the expectation of $\chi$-distribution with $k$ degree of freedom is

$$\sqrt{2}\,\frac{\Gamma((k+1)/2)}{\Gamma(k/2)}$$

the result follows.

# Appendix C: Technical results

## C.1. Proof of Proposition 4.8

Let $\tau_i$ be the $i$-th reflection jump time of $(z(t), e(t))$ for $i \ge 1$, and let $\tau_0 = 0, z(0) = z_0$. Let

$$\omega_n = \tau_n + 2\sum_{m=1}^{n-1}(-1)^m\tau_{n-m} + (-1)^{n+1}z_0, \quad \theta_n = \arctan\omega_n \;\; (n = 1, 2, \ldots). \tag{C.1}$$

Figure 1 illustrates the relation of the variables when $\alpha = \beta = 1$. In this case, $z(t)$ is the distance from the tangency point on a line segment to the process $y_{\mathrm{L}}(t)$.

**Lemma C.1.** *Assume that $\alpha = \beta = 1$. Then*

$$z(\tau_n -) = \omega_n \;\; (n \in \mathbb{N}) \tag{C.2}$$

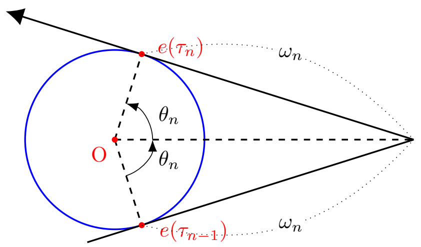


Figure 1: Relation among $\omega_n, \tau_n$ and $\theta_n$ when $\alpha = \beta = 1$.

*are independent and identically distributed and* $\mathbb{P}(w_n > x) = \exp(-x^2/2)$ *for* $x > 0$. *Also,*

$$\arccos(e(\tau_n)^\top e(\tau_{n-1})) = 2\theta_n \ (n = 1, 2, \ldots).$$

*In particular,*

$$\arccos(e(\tau_n)^\top e(0)) = 2\sum_{k=1}^{n} \theta_k \ (n = 1, 2, \ldots).$$

**Proof.** The process $z$ is completely determined by the stopping times. In particular, we have

$$z(\tau_n-) = \begin{cases} -z(\tau_{n-1}-) + (\tau_n - \tau_{n-1}) & n \geq 2 \\ z_0 + \tau_1 & n = 1. \end{cases}$$

since $z'(t) = 1$ for $t \neq \tau_n$ $(n = 1, 2, \ldots)$ and $z(\tau_n) = -z(\tau_n-)$. See Figure 2. Therefore, by inductive argument, we have $z(\tau_n-) = \omega_n$. Since $w_n$ denotes the time elapsed between the moment when $z(t)$ hits zero at time $t = \tau_{n-1} + z(t_{n-1})$ and the subsequent jump, and $z(t)_+$ represents the intensity function, we can draw the following conclusion:

$$\mathbb{P}(w_n > x) = \exp\left(-\int_0^x y \, \mathrm{d}y\right) = \exp(-x^2/2).$$

Thus the first claim follows. For the second claim, at the jump time $\tau_n$,

$$(27) \quad \Longrightarrow e(\tau_n)^\top e(\tau_n-) = b(z(\tau_n-), e(\tau_n-))^\top e(\tau_n-) = \frac{1 - z(\tau_n-)^2}{1 + z(\tau_n-)^2}.$$

Therefore

$$e(\tau_n)^\top e(\tau_{n-1}) = e(\tau_n)^\top e(\tau_n-) = \frac{1 - \omega_n^2}{1 + \omega_n^2} = \frac{1 - \tan\theta_n^2}{1 + \tan\theta_n^2} = \cos 2\theta_n.$$

Thus the second claim follows. The last claim follows from the fact that the process $y_{\mathrm{L}}(t)$ keeps its orientation. □

Let $P_t$ be the Markov semigroup of $H$.

**Lemma C.2.** *Assume that* $\alpha = \beta = 1$. *There is a coupling of measures* $P_t((z_0, e_0), \cdot)$ *and* $P_t((z_0^*, e_0^*), \cdot)$ *such that the first hitting time* $T_{D_0}$ *of*

$$D_0 = \{(z, e, z^*, e^*) \in (\mathbb{R} \times \mathbb{S})^2 : z = z^* = 0\}$$

*is finite with positive probability.*

**Proof.** Let $(z(t), e(t))$ and $(z^*(t), e^*(t))$ be the realisation of the coupling. The process $z$ is completely determined by the stopping times. In particular, as described in Figure 2,

$$z(t) = \begin{cases} t + z_0 & t \in [0, \tau_1) \\ t - (z_0 + 2\tau_1) & t \in [\tau_1, \tau_2) \end{cases} \quad \Longrightarrow \quad z(\xi) = 0, \text{ where } \xi = z_0 + 2\tau_1$$

Similarly, $z^*(\xi^*) = 0$, where $\xi^* = z_0^* + 2\tau_1^*$.

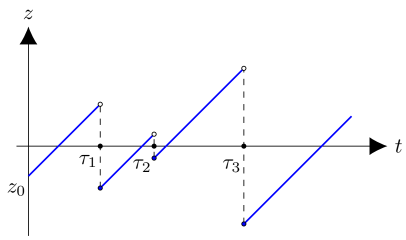


Figure 2: Path of $z(t)$ when $\alpha = \beta = 1$

We begin by defining $\mathbb{Q}$ as the maximal coupling of $\xi$ and $\xi^*$. Using this coupling, we construct a coupling of Markov processes, denoted by $\mathbb{P}$, by taking $(\xi, \xi^*) \sim \mathbb{Q}$ along with the conditionally independent realisations of stopping times given $\xi$ and $\xi^*$. From this construction, we obtain

$$\mathbb{P}\left(T_{D_0} < \infty\right) \;\geq\; \mathbb{P}(\xi = \xi^*) = \mathbb{Q}(\xi = \xi^*) = 1 - \|\mathcal{L}(\xi) - \mathcal{L}(\xi^*)\|_{\mathrm{TV}}.$$

The left-hand side equals to 0 if and only if the laws of $\xi$ and $\xi^*$ are mutually singular. However, since $\tau_1$ has a positive probability density on $[(-z_0)+, \infty)$, it follows that the random variable $\xi$ has a positive probability density on $[|z_0|, \infty)$, and similarly, $\xi^*$ has a positive probability density on $[|z_0^*|, \infty)$. Thus, the laws of $\xi$ and $\xi^*$ cannot be mutually singular, implying that the stopping time $T_{D_0}$ is finite with positive probability." □

**Lemma C.3.** *Assume that* $\alpha = \beta = 1$. *If* $e_0 + e_0^* \neq 0$, *there is a coupling of measures* $P_t((0, e_0), \cdot)$ *and* $P_t((0, e_0^*), \cdot)$ *such that the first hitting time* $T_D$ *of*

$$D = \{(z, e, z^*, e^*) \in (\mathbb{R} \times \mathbb{S})^2 : (z, e) = (z^*, e^*)\}$$

*is finite with positive probability.*

**Proof.** The process $z$ starting from $z(0) = 0$ satisfies

$$z(t) = \begin{cases} t & t \in [0, \tau_1) \\ t - 2\tau_1 & t \in [\tau_1, \tau_2) \\ t - 2(\tau_2 - \tau_1) & t \in [\tau_2, \tau_3) \end{cases} \implies z(\xi) = 0, \text{ where } \xi = 2(\tau_2 - \tau_1) \in [\tau_2, \tau_3). \tag{C.3}$$

Similarly, $z^*(\xi^*) = 0$ for $\xi^* = 2(\tau_2^* - \tau_1^*)$. Let $\epsilon = \arccos((e_0^*)^\top e_0)$ be the angle between the initial tangency points of two Markov processes. Without loss of generality, we can assume that $\epsilon \in (0, \pi)$. By Lemma C.1, the angle of $e(\xi)$ and $e^*(\xi^*)$ from $e(0)$ are twice of

$$\theta = \theta_1 + \theta_2, \quad \theta^* = \theta_1^* + \theta_2^* + \epsilon/2$$

where $\theta_n$ is defined in (C.1), and $\theta_n^*$ is as in (C.1), replacing $\tau_j$ by $\tau_j^*$. Thus

$$(\xi, \theta) = (\xi^*, \theta^*) \implies (z(\xi), e(\xi)) = (z^*(\xi), e^*(\xi)) \implies T_D < \infty.$$

As in the previous lemma, the proof will be completed if we can show that the laws of $(\xi, \theta)$ and $(\xi^*, \theta^*)$ are not mutually singular.

By (C.1) and (C.2),

$$\begin{cases} (\xi/2) = \omega_1 + \omega_2, \\ (\xi^*/2) = \omega_1^* + \omega_2^*, \end{cases} \qquad \begin{cases} \theta = \arctan \omega_1 + \arctan \omega_2, \\ \theta^* = \arctan \omega_1^* + \arctan \omega_2^* + \epsilon/2 \end{cases}$$

where $\omega_n = z(\tau_n -)$ and $\omega_n^* = z^*(\tau_n^* -)$. Both $(w_n)_n$ and $(w_n^*)_n$ are independent and identically distributed with positive probability density on $\mathbb{R}_+$. Thus, conditioned on $\xi$ and $\xi^*$, the variables $x = \omega_1/(\omega_1 + \omega_2)$ and $x^* = \omega_1^*/(\omega_1^* + \omega_2^*)$ are independent and identically distributed and have positive probability distribution function on the interval $[0, 1]$.

For given $\xi$ the map

$$f(x) = \arctan(x\xi/2) + \arctan((1 - x)\xi/2) \tag{C.4}$$

is symmetric about $x = 1/2$, and it is monotone increasing in the interval $[0, 1/2]$ since $f'(s) = (\xi/2)/(1 + (x\xi/2)^2) - (\xi/2)/(1 + ((1 - x)\xi/2)^2) > 0$. Thus

$$\arctan \xi/2 = f(0) \le f(x) \le f(1/2) = 2 \arctan \xi/4.$$

Therefore $\theta = f(x)$ has a positive probability density function on $[\arctan \xi/2, 2 \arctan \xi/4]$, and $\theta^* = \epsilon + f(x^*)$ has a positive probability density function on $[\epsilon/2 + \arctan \xi/2, \epsilon/2 + 2 \arctan \xi/4]$. These measures are not mutually singular if

$$\epsilon/2 + \arctan \xi/2 < 2 \arctan \xi/4.$$

The function $g(\xi) = 2 \arctan \xi/4 - \arctan \xi/2$ is a monotone increasing function and $\sup_{\xi \in \mathbb{R}_+} g(\xi) = \pi/2$. Thus if $\epsilon < \pi$, then the laws of $\theta$ and $\theta^*$ given $\xi = \xi^*$ are not mutually singular if we take $\xi = \xi^*$ large enough. Thus $T_D$ is finite with a positive probability. □

**Lemma C.4.** *Assume that $\alpha = \beta = 1$. If $e + e^* = 0$, there is a coupling of measures $P_t((0, e_0), \cdot)$ and $P_t((0, e_0^*), \cdot)$ such that the first hitting time $T_D$ of*

$$D_0' = \{(z, e, z^*, e^*) \in (\mathbb{R} \times \mathbb{S})^2 : (z, e) = (z^*, e^*), e + e^* \ne 0\}$$

*is finite with positive probability.*

**Proof.** Let $\theta_n$ and $\omega_n$ as in (C.1), and let $\theta_n^*$ and $\omega_n^*$ be the same replacing $\tau_n$ by $\tau_n^*$. Then

$$\xi := 2(\tau_2 - \tau_1) = 2(\omega_1 + \omega_2),\ \xi^* := 2\tau_1^* = 2\omega_1 \overset{(C.3)}{\Longrightarrow} z(\xi) = z^*(\xi^*) = 0.$$

Let $\mathbb{Q}$ be maximal coupling of the laws of $\xi$ and $\xi^*$. Then $\mathbb{Q}(\xi = \xi^*) > 0$. The coupling of Markov processes, denoted by $\mathbb{P}$, is constructed by $(\xi, \xi^*) \sim \mathbb{Q}$ together with the conditionally independent realisations of stopping times given $\xi$ and $\xi^*$. The variable $x = \omega_1/(\omega_1 + \omega_2)$ has a continuous probability density function on $[0, 1]$ under $\mathbb{P}$ given $\xi$ and $\xi^*$.

On the other hand, by Lemma C.1,

$$\arccos e(\xi)^\top e(0) = 2\theta_2 + 2\theta_1,\ \arccos e^*(\xi^*)^\top e^*(0) = 2\theta_1^*,$$
$$\overset{\text{if } \xi=\xi^*}{\Longrightarrow} \quad \arccos e(\xi)^\top e^*(\xi) = 2(\theta_1 + \theta_2 - \theta_1^*) + \pi.$$

Since the arctangent function is a subadditive function on $\mathbb{R}_+$, we have

$$\begin{aligned}\xi = \xi^* \implies \theta_1 + \theta_2 - \theta_1^* &\overset{(C.1)}{=} \arctan \omega_1 + \arctan \omega_2 - \arctan \omega_1^* \\ &= \arctan(x\xi/2) + \arctan((1-x)\xi/2) - \arctan(\xi/2) > 0 \\ &\implies e(\xi) + e^*(\xi) \neq 0\end{aligned}$$

where we used the fact that $f(x)$ defined in (C.4) is monotone increasing. Thus $\xi = \xi^* \implies (z(\xi), e(\xi), z^*(\xi), e^*(\xi)) \in D_0'$. Hence $\mathbb{P}(T_{D_0'} < \infty) \geq \mathbb{Q}(\xi = \xi^*) > 0$. □

**Proof of Proposition 4.8.** Let $w(t) = (z(t), e(t), z^*(t), e^*(t))$ and let $(\mathcal{F}_t)$ be the filtration. We assume $\alpha = \beta = 1$. This is always possible by state scaling and time scaling. Without loss of generality, we can assume that the process $z$ is counter clockwise and all angles in this proof will be measured in this orientation.

We use the couplings in Lemmas C.2, C.3, and C.4, as described in equation (C.5). Specifically, we first use the coupling in Lemma C.3 for $(z, e) \in \mathbb{R} \times \mathbb{S}$ until it hits $D_0$. If it is in $(D_0')^c$, we then use Lemma C.2 until it hits $D_0'$. Finally, from $D_0$ until it reaches $D$, we use the coupling in Lemma C.4:

$$(z, e) \overset{\text{Lemma } C.3}{\Longrightarrow} D_0 \quad (\text{if } e + e' = 0 \overset{\text{Lemma } C.4}{\Longrightarrow} D_0') \overset{\text{Lemma } C.2}{\Longrightarrow} D \tag{C.5}$$

By Markov property, the constructed probability measure satisfies $\mathbb{P}(T_D < \infty) > 0$. Hence, by modifying the processes so that they are coincides after $t = T_D$, we can show that there exists $T > 0$ such that $0 < \mathbb{P}(T_D < T) = 1 - \|P_T((z, e), \cdot) - P_T((z^*, e^*), \cdot)\|_{\mathrm{TV}}$. Therefore, the claim follows. □

## C.2. Two dimensional analysis of the Zig-Zag sampler

Let $e_\alpha(x) = \exp(-\alpha x^2/2)$ and define functions $E_\alpha$ and $\overline{E}_\alpha$ as follows:

$$E_\alpha(x) = \int_0^x e_\alpha(y)\mathrm{d}y, \quad \overline{E}_\alpha(x) = \int_x^\infty e_\alpha(y)\mathrm{d}y$$

for $\alpha \in \mathbb{R}$. Note that $e_\alpha(x)' = -\alpha x e_\alpha(x)$ and $E_\alpha(+\infty) = \overline{E}_\alpha(0) = \sqrt{\pi/2\alpha}$ for $\alpha > 0$. Suppose for the function $h : \mathbb{R} \to \mathbb{R}$, $h(x)e_\alpha(x)$ is integrable. For $x \in I = (0, \infty)$ or $(-\infty, 0)$, and for a differentiable

function $f : I \to \mathbb{R}$,

$$\begin{aligned} f'(x) - \alpha x f(x) = h(x) \quad &\Longrightarrow \quad (e_\alpha(x)\ f(x))' = e_\alpha(x)\ h(x) \\ &\Longrightarrow \quad f(x) = e_\alpha(x)^{-1} \left( C + \int_0^x e_\alpha(y)\ h(y) \mathrm{d}y \right) \end{aligned}$$

where $C$ is a constant. We denote the solution by $F(\alpha, h)(x)$, which is indeterminate up to the constant $C \in \mathbb{R}$. We write $f \equiv_a g$ if $f(x) - g(x) = C e_\alpha(x)^{-1}$ for some $C \in \mathbb{R}$.

**Lemma C.5.** *Let* $\alpha \neq \beta$ *and* $\alpha, \beta \neq 0$. *Then* $F(\alpha, af + bg) \equiv_\alpha aF(\alpha, f) + bF(\alpha, g)$ *for* $a, b \in \mathbb{R}$ *and* $\mathcal{N}(0, \alpha^{-1})$*-integrable functions* $f$ *and* $g$. *Moreover,*

$$F(\alpha, 1) \equiv_\alpha e_\alpha(x)^{-1} E_\alpha(x), \quad F(\alpha, x) \equiv_\alpha -\alpha^{-1}$$

*and*

$$F(\alpha, x^2) \equiv_\alpha -\alpha^{-1} x + \alpha^{-1} F(\alpha, 1).$$

*Also,*

$$F(\alpha, xF(\beta, 1)) \equiv_\alpha \frac{1}{\alpha - \beta}(F(\alpha, 1) - F(\beta, 1)),\ F(\alpha, x e_\beta(x)^{-1}) \equiv_\alpha -\frac{1}{\alpha - \beta} e_\beta(x)^{-1}.$$

**Lemma C.6.** *For* $0 < \beta < \alpha$,

$$\begin{aligned} I(\alpha, \beta) &= \int_0^\infty E_\beta(x) e_\alpha(x) \mathrm{d}x = (\alpha\beta)^{-1/2} \arctan \sqrt{\frac{\beta}{\alpha}} \\ I(\alpha, -\beta) &= \int_0^\infty E_{-\beta}(x) e_\alpha(x) \mathrm{d}x = (\alpha\beta)^{-1/2} \operatorname{arctanh} \sqrt{\frac{\beta}{\alpha}} \\ \overline{I}(-\beta, \alpha) &= \int_0^\infty \overline{E}_\alpha(x) e_{-\beta}(x) \mathrm{d}x = (\alpha\beta)^{-1/2} \operatorname{arctanh} \sqrt{\frac{\beta}{\alpha}}. \end{aligned}$$

**Proof.** We have

$$\begin{aligned} I(\alpha, \beta) &= \int_0^\infty \int_0^\infty 1_{\{y \le x\}} e_\beta(y) e_\alpha(x) \mathrm{d}x \mathrm{d}y \\ &= (\alpha\beta)^{-1/2} \int_0^\infty \int_0^{\pi/4} 1_{\{\tan\theta \le \sqrt{\beta/\alpha}\}} \exp(-r^2/2) \mathrm{d}\theta\ r\ \mathrm{d}r \\ &= (\alpha\beta)^{-1/2} \arctan \sqrt{\frac{\beta}{\alpha}} \end{aligned}$$

where we consider variable transformation $x = \alpha^{-1/2} r \cos\theta$, $y = \beta^{-1/2} r \sin\theta$. Under the same transformation, we have

$$\begin{aligned} I(\alpha, -\beta) &= \int_0^\infty \int_0^\infty 1_{\{y \le x\}} e_{-\beta}(y) e_\alpha(x) \mathrm{d}x \mathrm{d}y \\ &= (\alpha\beta)^{-1/2} \int_0^\infty \int_0^{\pi/4} 1_{\{\tan\theta \le \sqrt{\beta/\alpha}\}} \exp(-((\cos\theta)^2 - (\sin\theta)^2) r^2/2) \mathrm{d}\theta\ r\ \mathrm{d}r. \end{aligned}$$

Since $\sin\theta < \cos\theta$ when $0 < \theta < \pi/4$, we have

$$I(\alpha,-\beta) = (\alpha\beta)^{-1/2}\int_0^{\arctan\sqrt{\beta/\alpha}} \frac{1}{(\cos\theta)^2 - (\sin\theta)^2}\mathrm{d}\theta$$
$$= (\alpha\beta)^{-1/2}\int_0^{\sqrt{\beta/\alpha}} \frac{1}{1-x^2}\mathrm{d}x$$

where we consider variable transformation $x = \tan\theta$. Therefore

$$(\operatorname{arctanh} z)' = \frac{1}{1-z^2} \implies I(\alpha,-\beta) = (\alpha\beta)^{-1/2}\operatorname{arctanh}\sqrt{\frac{\beta}{\alpha}}$$

where $\operatorname{arctanh} z = (\log(1+z) - \log(1-z))/2$. Finally, we have

$$\bar{I}(-\beta,\alpha) = \int_0^\infty\int_0^\infty 1_{\{x\le y\}} e_\alpha(y) e_{-\beta}(x)\mathrm{d}x\mathrm{d}y = I(\alpha,-\beta).$$

□

Let $\mathcal{F}_1, \mathcal{F}_2$ be operations such that

$$\mathcal{F}_1 f(x,i,j) = f(x,-i,j), \quad \mathcal{F}_2 f(x,i,j) = f(x,i,-j) \ (x\in\mathbb{R}, i,j\in\{-1,+1\}).$$

**Proposition C.7.** *Let $g : \{0,1\} \to \mathbb{R}$, and let*

$$\alpha(i,j) = \frac{p}{ip+jq},\ \beta(i,j) = \frac{q}{ip+jq}$$

*for $p,q\in\mathbb{R}$ such that $|p|\neq|q|$. Consider an equation*

$$\mathcal{G} f(x,i,j) = g_{|i-j|}$$

*for $x\in I$ and $i,j\in\{-1,+1\}$ where*

$$\mathcal{G} f(x,i,j) = f'(x,i,j) + x\ \{i_+\,\alpha(i,j)\ (\mathcal{F}_1 - \mathrm{id}) f(x,i,j) + j_+\,\beta(i,j)\ (\mathcal{F}_2 - \mathrm{id}) f(x,i,j)\}.$$

*A solution is given by $f(x,-,-) = xg_0 + C$ and*

$$\begin{aligned} f(x,+,-) &= f(x,-,-) + F(p/(p-q),1)(g_1 - g_0),\\ f(x,-,+) &= f(x,-,-) + F(q/(q-p),1)(g_1 - g_0) \end{aligned} \tag{C.6}$$

*and*

$$f(x,+,+) \equiv_1 f(x,-,-) + \frac{p-q}{p+q}\ (F(q/(q-p),1) - F(p/(p-q),1))(g_1 - g_0) \tag{C.7}$$

*for $C\in\mathbb{R}$.*

**Proof.** We solve the equation $\mathcal{G} f(x,i,j) = g(x,i,j)$ by solving four equations corresponding to $(i,j)\in\{-1,+1\}^2$ sequentially. For the simplest case,

$$(i,j) = (-,-) \implies f' = g_0 \implies f(x,-,-) = x\ g_0 + C.$$

For the cases where one of $i$ or $j$ is positive, we have

$$(i,j)=(+,-) \implies f'-x\alpha\, f=g_1-x\alpha\,\mathcal{F}_1 f \implies f\equiv_\alpha F(\alpha,g_1-x\alpha\mathcal{F}_1 f),$$
$$(i,j)=(-,+) \implies f'-x\beta\, f=g_1-x\beta\,\mathcal{F}_2 f \implies f\equiv_\beta F(\beta,g_1-x\beta\mathcal{F}_2 f).$$

Observe that $\mathcal{F}_1 f$ and $\mathcal{F}_2 f$ in the right-hand side of the above are $xg_0+C$. By Lemma C.5, (C.6) follows. Finally,

$$(i,j)=(+,+)\Rightarrow f'-x\,f=g_0-x(\alpha\mathcal{F}_1 f+\beta\mathcal{F}_2 f)\Rightarrow f\equiv_1 F(1,g-x(\alpha\mathcal{F}_1 f+\beta\mathcal{F}_2 f)).$$

Thus,

$$\begin{aligned} f(x,+,+) &\equiv_1 g_0F(1,1)-\frac{p}{p+q}F(1,xf(x,-,+))-\frac{q}{q+p}F(1,xf(x,+,-)) \\ &\equiv_1 g_0F(1,1)-g_0F(1,x^2)-CF(1,x) \\ &\quad -\frac{p}{p+q}(g_1-g_0)F\left(1,xF\left(\frac{q}{q-p},1\right)\right) \\ &\quad -\frac{q}{q+p}(g_1-g_0)F\left(1,xF\left(\frac{p}{p-q},1\right)\right). \end{aligned}$$

This proves (C.7) by Lemma C.5. □

If $x\ge 0$ and if $i|\sin\theta|+j|\cos\theta|\neq 0$, then

$$\begin{cases} v_1:=i\ \mathrm{sgn}(\sin\theta) \\ v_2:=j\ \mathrm{sgn}(\cos\theta) \\ p:=|\sin\theta| \\ q:=|\cos\theta| \end{cases} \implies \begin{cases} i_+\ \alpha(i,j)\ x=\dfrac{i_+\ |\sin\theta|\ x}{i\ |\sin\theta|+j\ |\cos\theta|}=\dfrac{(v_1x\sin\theta)_+}{v_1\sin\theta+v_2\cos\theta} \\[2ex] j_+\ \beta(i,j)\ x=\dfrac{j_+\ |\cos\theta|\ x}{i\ |\sin\theta|+j\ |\cos\theta|}=\dfrac{(v_2x\cos\theta)_+}{v_1\sin\theta+v_2\cos\theta} \end{cases}$$

For $x\ge 0$, the solution $\chi(x,v)$ of (4) corresponds to the case where

$$g(|i-j|)=\frac{-v_1\cos\theta+v_2\sin\theta}{v_1\sin\theta+v_2\cos\theta}=\frac{-iq+jp}{ip+jq}\ \mathrm{sgn}(\sin\theta\cos\theta).$$

The generator $\mathcal{L}_0$ is ergodic, and so the solution $\chi(x,v)$ of the Poisson equation is unique up to a constant. Therefore, $\chi(x,v)=-\chi(-x,-v)+C$ for some $C\in\mathbb{R}$ since $-\chi(-x,-v)$ is also a solution. However this implies $\chi(0,v)=-\chi(0,-v)+C=\chi(0,v)+2C$ and $C=0$. Therefore,

$$\chi(x,v)=-\chi(-x,-v). \tag{C.8}$$

By (C.8) of $\chi$, we have

$$\Omega=\sum_{v_1,v_2\in\{-1,+1\}}\int_0^\infty \chi(x,v_1,v_2)\phi(x)\mathrm{d}x\ (v_1\cos\theta-v_2\sin\theta). \tag{C.9}$$

A solution $F(\alpha,1)$ is determined up to a constant times $e_\alpha^{-1}$. However we need to fix the constant so that $\chi(x,v)$ is $\mathcal{N}(0,1)$-integrable and it satisfies (C.8) and continuity at $x=0$. In particular, $\chi(0,+,-)=$

$-\chi(0,-,+)$ and $\chi(0,-,-)=-\chi(0,+,+)$. After some calculation, for $x \geq 0$ we set

$$F(\alpha,1)=\begin{cases} e_\alpha^{-1}(x)(E_\alpha(x)-\overline{E}_{1-\alpha}(0)\ \dfrac{1-\alpha}{\alpha}) & \text{if } \alpha<0 \\ -e_\alpha^{-1}(x)\overline{E}_\alpha(x) & \text{if } 1<\alpha. \end{cases}$$

for $\alpha \notin [0,1]$ and $C=-F(\alpha,1)(0)\ (g_1-g_0)/2(1-\alpha)$ where $C$ is the constant in Proposition C.7. Here, we consider the equivalent relation in (C.7) as an equation. We have

$$\int_0^\infty F(\alpha,1)\phi(x)\mathrm{d}x=\frac{1}{\sqrt{2\pi}}\times\begin{cases} I(1-\alpha,\alpha)-\overline{E}_{1-\alpha}(0)^2\ \dfrac{1-\alpha}{\alpha} & \text{if } \alpha<0 \\ -\overline{I}(1-\alpha,\alpha) & \text{if } 1<\alpha. \end{cases}$$

**Proposition C.8.** *For $\theta \neq n\pi/4$ $(n=0,\dots,7)$, the value of $\Omega$ is expressed as (5).*

**Proof.** We evaluate the integrals

$$J(i,j)=\int_0^\infty \chi(x,i,j)\phi(x)\mathrm{d}x$$

where we omit $C$ in Proposition C.7 since it will be cancelled out in the integral in (C.9). Assume $x>0$. First we consider $p<q$, that is, $|\sin\theta|<|\cos\theta|$ case. In this case, $q/(q-p)>1$ and $p/(p-q)<0$ and by Lemma C.5, we have

$$\begin{aligned} J(-,-)&=\frac{1}{\sqrt{2\pi}}g_0 \\ J(+,-)&=\frac{1}{\sqrt{2\pi}}g_0+\frac{1}{\sqrt{2\pi}}(g_1-g_0)\left(I+\overline{E}_{q/(q-p)}(0)^2\frac{q}{p}\right) \\ J(-,+)&=\frac{1}{\sqrt{2\pi}}g_0-\frac{1}{\sqrt{2\pi}}(g_1-g_0)I \\ J(+,+)&=\frac{1}{\sqrt{2\pi}}g_0+\frac{1}{\sqrt{2\pi}}\frac{p-q}{p+q}(g_1-g_0)\left(-2I-\overline{E}_{q/(q-p)}(0)^2\frac{q}{p}\right), \end{aligned}$$

where $I=I(q/(q-p),p/(p-q))=(\operatorname{arctanh}\sqrt{p/q})(q-p)/\sqrt{pq}$. By (C.9), we have

$$\Omega=\sum_{i,j\in\{-,+\}}\delta(i,j)\int_0^\infty \chi(x,i,j)\phi(x)\mathrm{d}x$$

where $\delta(i,j)=v_1\cos\theta-v_2\sin\theta=(iq-jp)\ \mathrm{sgn}(\cos\theta\sin\theta)$. Therefore,

$$\begin{aligned} \Omega&=\frac{1}{\sqrt{2\pi}}(g_1-g_0)I\left\{\delta(+,-)-\delta(-,+)-2\delta(+,+)\frac{p-q}{p+q}\right\} \\ &\quad+\frac{1}{\sqrt{2\pi}}(g_1-g_0)\overline{E}_{q/(q-p)}(0)^2\ \frac{q}{p}\ \left\{\delta(+,-)-\frac{p-q}{p+q}\delta(+,+)\right\} \\ &=\frac{8}{\sqrt{2\pi}}\frac{(p^2+q^2)^2}{(p+q)^2(q-p)}I+\frac{\sqrt{2\pi}(p^2+q^2)^2}{p(p+q)^2}. \end{aligned}$$

Thus

$$\Omega = \frac{8}{\sqrt{2\pi}} \frac{\operatorname{arctanh}\sqrt{|\tan\theta|}}{(|\sin\theta| + |\cos\theta|)^2\sqrt{|\sin\theta\cos\theta|}} + \frac{\sqrt{2\pi}}{|\sin\theta|(|\sin\theta| + |\cos\theta|)^2}.$$

When $q < p$, similar calculation yields

$$\Omega = \frac{8}{\sqrt{2\pi}} \frac{\operatorname{arctanh}\sqrt{1/|\tan\theta|}}{(|\sin\theta| + |\cos\theta|)^2\sqrt{|\sin\theta\cos\theta|}} + \frac{\sqrt{2\pi}}{|\cos\theta|(|\sin\theta| + |\cos\theta|)^2}.$$

Hence the expression (5) follows. □

## C.3. Local law of large numbers

**Lemma C.9.** *Let $\xi$ be a stationary process with the stationary distribution $\mu$. For any $T > 0$ and $\mu$-integrable function $f$,*

$$\mathbb{E}\left[\sup_{0\le t\le T}\left|\frac{1}{T}\int_0^t f(\xi(t))\mathrm{d}t\right|\right] \le \mathbb{E}\left[\left|\frac{1}{S}\int_0^S f(\xi(t))\mathrm{d}t\right|\right] + \frac{S}{T}\,\mu(|f|).$$

**Proof.** Let $[x]$ be the integer part of $x > 0$. We consider dividing a closed interval with length $T$ into $[T/S]$ short intervals with length $S$ and a remainder interval with length $T - S\,[T/S]$. Applying this decomposition, we have

$$\left|\int_0^T f(\xi(t))\mathrm{d}t\right| \le \sum_{i=1}^{[T/S]}\left|\int_{(i-1)S}^{iS} f(\xi(t))\mathrm{d}t\right| + \left|\int_{T-S[T/S]} f(\xi(t))\mathrm{d}t\right|$$

By stationarity, applying above decomposition, we have

$$\mathbb{E}\left[\sup_{0\le t\le T}\left|\int_0^t f(\xi(t))\mathrm{d}t\right|\right] \le \left[\frac{T}{S}\right]\,\mathbb{E}\left[\left|\int_0^S f(\xi(t))\mathrm{d}t\right|\right] + S\,\mu(|f|).$$

Thus the claim follows from $[x] \le x$. □

# References

Ikeda, N. and Watanabe, S. (1989). *Stochastic Differential Equations and Diffusion Processes*, 2nd ed. North-Holland Mathematical Library 24. North-Holland Publishing Co., Amsterdam; Kodansha, Ltd., Tokyo. MR1011252.

Jacod, J. and Shiryaev, A. N. (2003). *Limit Theorems for Stochastic Processes.*, 2nd ed. Grundlehren der Mathematischen Wissenschaften. Springer-Verlag, Berlin.

Kurtz, T. G. (2011). Equivalence of stochastic equations and martingale problems. In *Stochastic Analysis 2010*, 113–130. Springer, Heidelberg. MR2789081. https://doi.org/10.1007/978-3-642-15358-7_6.

Pavliotis, G. A. (2014). *Stochastic Processes and Applications*. Springer New York. https://doi.org/10.1007/978-1-4939-1323-7.

Pavliotis, G. A. and Stuart, A. M. (2008). *Multiscale Methods: Averaging and Homogenization*. Texts in Applied Mathematics 53. Springer, New York.
